# Supplementary material for: Error-Corrected Eternal Lifetime Storage
Source: arXiv:2503.22355 source file (2025-03-28)
Supplement: Supplementary file 1 [file SM.pdf]

# Supporting information for Error-Corrected Eternal Lifetime Storage

Jie Ma<sup>1,2</sup>, Chu-Han Wang<sup>1,2</sup>, Xiao-Yun Xu<sup>1,2</sup>, Chang-Kun Shi<sup>5</sup>, Tian-Yu Zhang<sup>1,2</sup>, Ke Cheng<sup>1,2\*</sup>, Li Zhan<sup>3\*</sup>, Xian-Min Jin<sup>1,2,4,5\*</sup>

<sup>1</sup>Center for Integrated Quantum Information Technologies (IQIT), School of Physics and Astronomy and State Key Laboratory of Advanced Optical Communication Systems and Networks, Shanghai Jiao Tong University, Shanghai 200240, China

<sup>2</sup>Hefei National Laboratory, Hefei 230088, China

<sup>3</sup>State Key Laboratory of Advanced Optical Communication Systems and Networks, School of Physics and Astronomy, Shanghai Jiao Tong University, Shanghai, 200240, China

<sup>4</sup>TuringQ Co., Ltd., Shanghai 200240, China

<sup>5</sup>Chip Hub for Integrated Photonics Xplore (CHIPX), Shanghai Jiao Tong University, Wuxi 214000, China

\*E-mail: chengkek@sjtu.edu.cn

\*E-mail: lizhan@sjtu.edu.cn

\*E-mail: xianmin.jin@sjtu.edu.cn

The supplemental document includes details of the high-fidelity data writing and reading process based on femtosecond laser direct writing and error correction code, model diagram of femtosecond laser direct writing and birefringence microscope reading device, femtosecond laser modification to form anisotropic nanostructures, trade-off between storage information capacity and redundancy length, display of data classification effects, display of label maps for 256 categories, measurement of real data based on birefringence microscopy system, multi-layer data simulation diagram based on real data, the Encoding and Decoding Principle of Reed-Solomon Error Correction Algorithm.

## 1 High-fidelity data writing and reading process based on femtosecond laser direct writing and error correction code.

The flowchart of using femtosecond laser direct writing system for data storage is shown in Figure. 1. Original information to be stored is converted into binary data according to the rules of the ASCII code, and add redundant information according to the selected RS rules. The obtained binary data is converted into five-dimensional data. The conversion rules depend on the requirements and settings for direct writing of the polarization and power of the femtosecond laser in the five-dimensional data. Laser direct writing is then conducted on fused silica, guided by designated parameters. The operation of data readout process utilizing a birefringent microscope is elucidated in Figure. 2. The data images taken by the microscope are processed using deep learning methods, especially the TPH-YOLOv5 recognition algorithm and VGG16 classification algorithm, to retrieval the storage data. After data is read out, the original data can be recovered according to RS decoding principle.

TPH-YOLOv5 is a one-stage object detection algorithm that provides a conspicuous advantage in terms of object recognition speed. Given the multi-dimensional encoding of retardance of data, there are multiple data points that require optical frame selection to achieve accurate detection of objects of varying sizes.

Firstly, we use a birefringent microscope to take a batch of data images with a resolution of  $2048 \times 2048$  pixels. In order to enhance the model's generalization ability and prevent potential overfitting issues during subsequent training, we employ data augmentation techniques such as random rotation, scale transformation, and HSV enhancement, based on the shape and color features of the data points. The optimizer used for training is AdamW, which can automatically adjust the learning rate and greatly improve the training speed. After getting the initial model, we use TPH-YOLOv5 to crop and extract small images of  $32 \times 32$  pixels with the same label from each large image as the training sets.

On account of the low accuracy and efficiency of TPH-YOLOv5 classifier, we pack small images by category and feed them into VGG16 for training. VGG16 performs well in neural network classification algorithm due to its three-layer fully connected architecture. In particular, it utilizes multiple consecutive  $3 \times 3$  convolution kernels to improve classification results over larger convolution kernels. By leverag-

ing multilayer nonlinear layers, it can achieve a greater depth of network to learn more complex patterns and distinguish between different types of points accurately.

We use the Focal loss function to ensure the recognition of samples that are difficult to distinguish and continue to use the AdamW optimizer for training. For each type of sample, we have 1600 small images for training, while 1280 of them are used for training, and the remaining 320 points are used for result inspection to verify the effectiveness of VGG16 network training. Finally, we test a substantial amount of real data under the trained VGG16 neural network and compare it with the original data to obtain its recognition accuracy data.

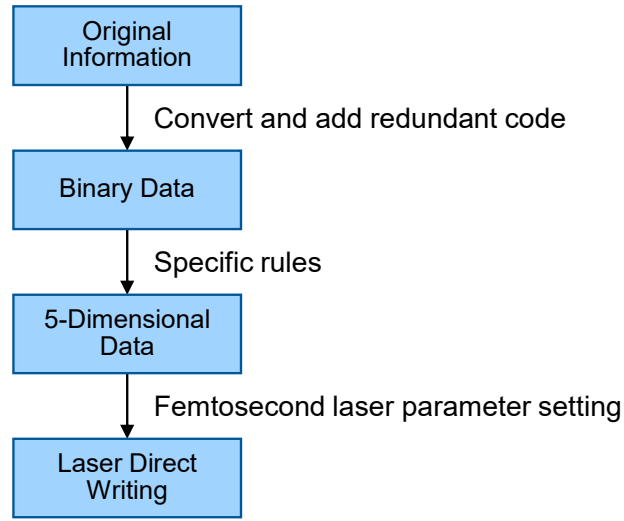

Figure 1: Data writing process using femtosecond laser.

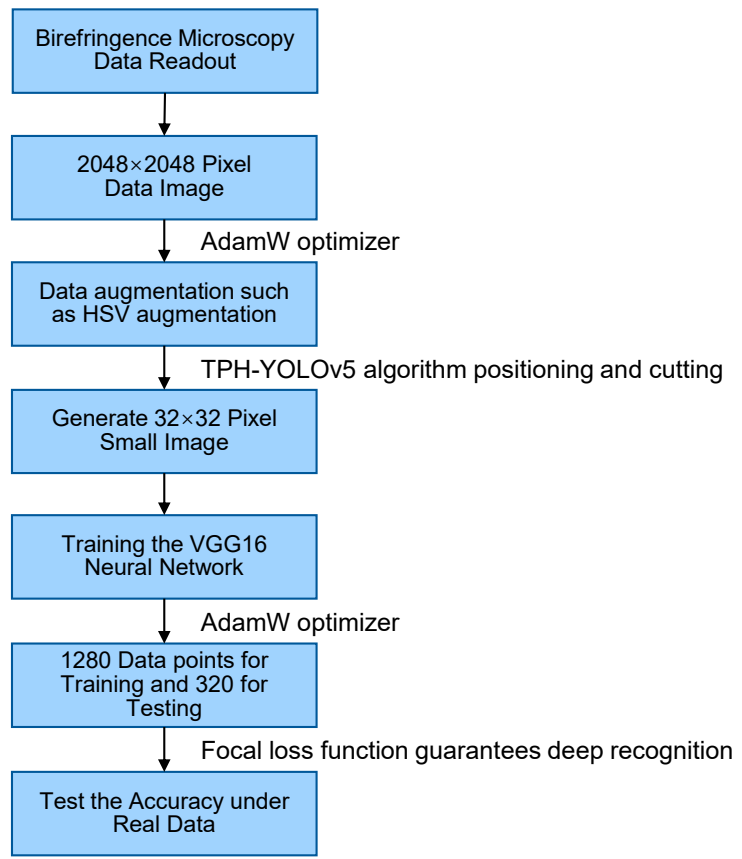

Figure 2: Data reading, processing and recovery process using birefringence microscopy system.

## 2 Model diagram of femtosecond laser direct writing and birefringence microscope reading device.

The model diagram of the femtosecond laser direct writing data writing device is shown in Figure 3. The Femtosecond laser direct writing system for high-precision data optical storage consists of the following parts. Femtosecond laser source generates laser beam with extremely short pulse durations, which have the characteristics of high peak power and low thermal effects. After passing through optical components such as lenses, attenuator, polarizer, etc., the laser is focused on the interior of the storage medium for modification. Commonly used storage media include fused silica, which offers excellent heat resistance and chemical stability, is suitable for high-power laser direct writing processes. The formed nanograting structure with data information theoretically has a permanent life. A high-precision motion control system (Aerotech AL1500) is used to control the movement of storage media to achieve precise writing of data. The CIS(CMOS Image Sensor) camera plays a critical role in the femtosecond laser direct writing system: a) Real-Time Monitoring: It captures high-resolution images of the laser processing area in real time. b) Precision Control: These images are used to monitor the interaction between the femtosecond laser and the material, ensuring that modifications occur precisely in the intended locations. c) Quality Assurance: The camera helps detect potential deviations or errors during the writing process, allowing for corrective measures to maintain high-quality data writing.

The model diagram of the birefringence microscope reading device is shown in Figure 4. The birefringence microscopy system uses the birefringence properties inside the storage medium to observe materials, thereby achieving accurate data extraction. The light source of the system we use is a high-brightness white light source passing through a 530nm filter to meet the brightness requirements of microscopic observation. The polarizing device of the system includes polarizing plate and polarizer. Polarizing plate is used to generate polarized light sources, while polarizer is used to adjust and control the polarization direction of light. These components can be electrically controlled to change the polarization state of light to achieve different observation modes of the sample. The objective lens has the function of amplifying and focusing light and has high resolution to produce a clear  $2048 \times 2048$  microscopic data image on the CCD, providing material for subsequent data recovery.

In future work, we consider integrating the femtosecond laser direct writing system with the birefringence microscope system to achieve simultaneous writing and reading of data.

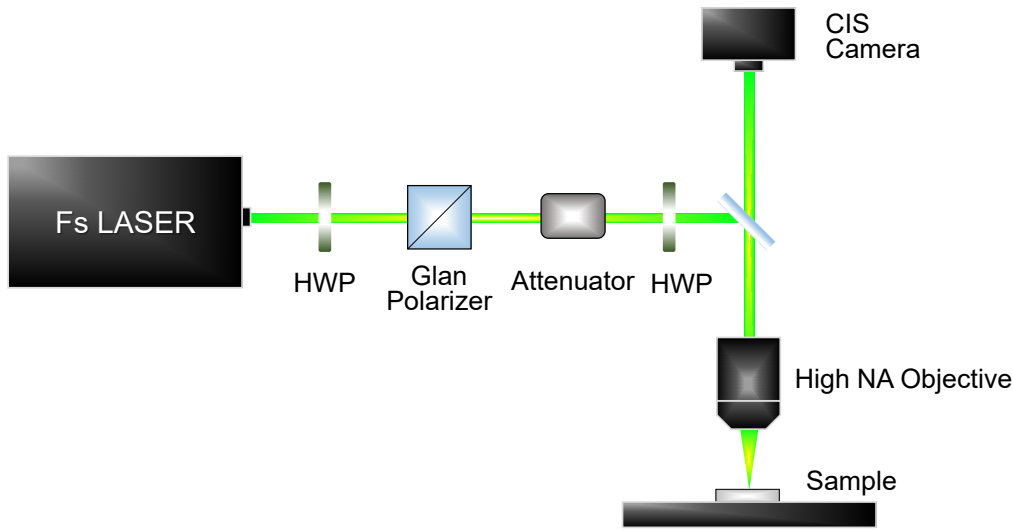

Figure 3: Schematic diagram of femtosecond laser data writing device.

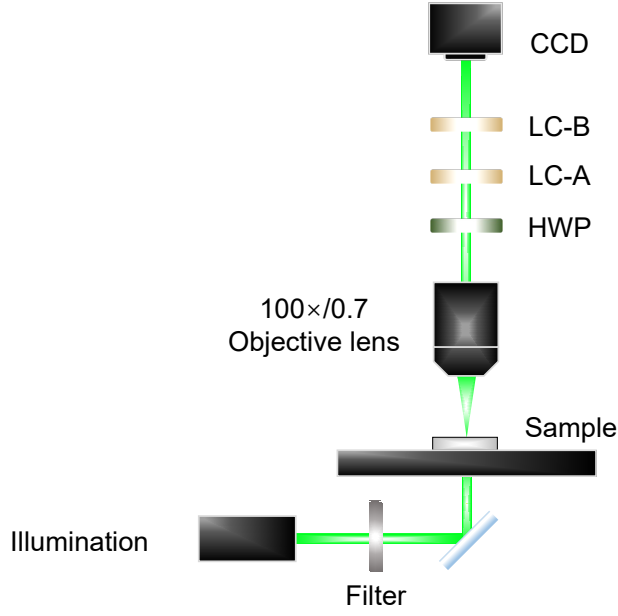

Figure 4: Schematic diagram of the data reading device of the birefringence microscope.

### 3 Femtosecond laser modification to form anisotropic nanostructures.

When femtosecond laser generates anisotropic structures in fused silica, the laser parameters have a significant impact on the modification of its structural materials, and the formation of nanogratings also has a corresponding parameter window. Since we want to perform multi-dimensional encoding based on the retardance of the nanogratings, it is important to choose an appropriate distinguishable interval. We tested the relationship between the laser power and the number of pulses for single point direct writing and the measured retardance. The retardance of the formed structure increases as laser power and the number of pulses grow, as shown in Figure 5 and Figure 6. Within an acceptable error range, the influence of laser polarization on the retardance is negligible. However, it is easy to see that it is more obvious for power changes which are shown in Table 1-4.

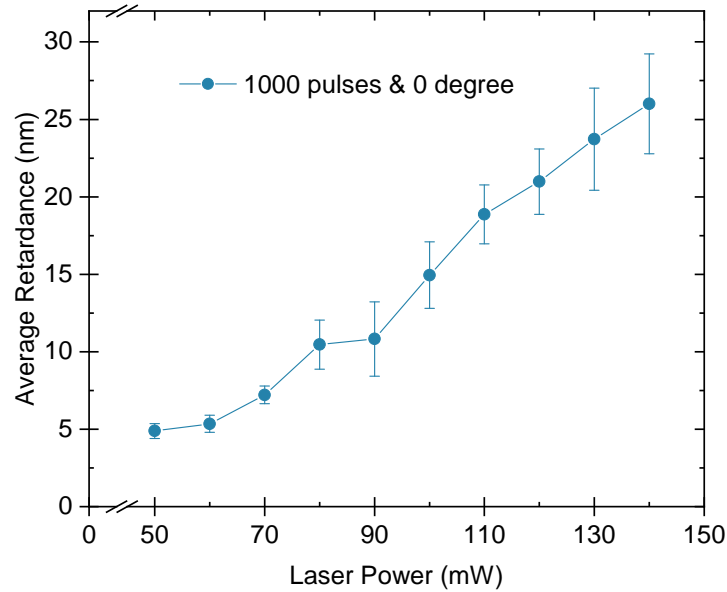

Figure 5: The relationship between the retardance of nanograting and the power of femtosecond laser(Single point write using 1000 pulses).

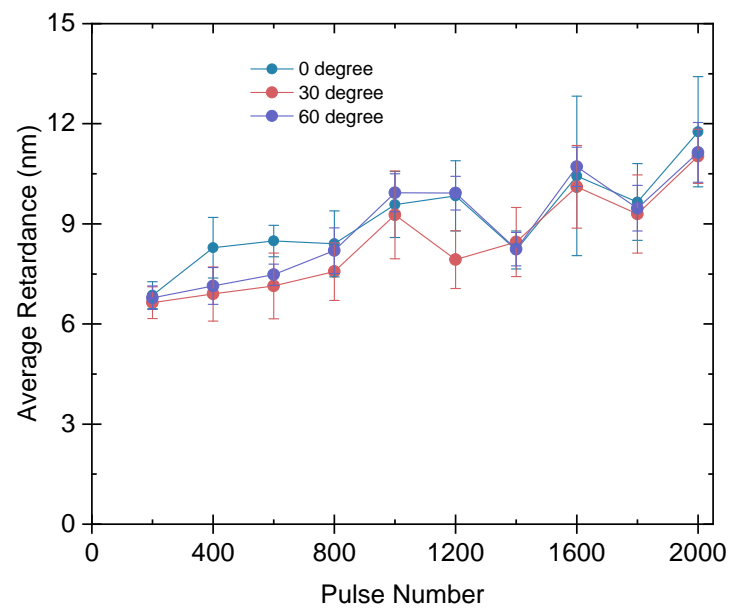

Figure 6: The relationship between the retardance of nanograting and the pulse of femtosecond laser(The laser power is 80mW).

Table 1: The relationship between laser power and retardance.

| Laser Power(mW) |       | Parts of Retardance(nm) |       |       |       |       |       |       |       |
|-----------------|-------|-------------------------|-------|-------|-------|-------|-------|-------|-------|
| 50              | 5.48  | 4.53                    | 4.63  | 4.68  | 5.79  | 4.72  | 5.22  | 5.22  | 4.37  |
| 60              | 4.82  | 4.72                    | 5.28  | 4.86  | 5.41  | 5.62  | 5.70  | 4.31  | 5.23  |
| 70              | 6.72  | 6.83                    | 6.84  | 6.76  | 7.19  | 7.22  | 6.66  | 6.74  | 7.38  |
| 80              | 9.36  | 8.96                    | 12.22 | 10.41 | 10.37 | 9.50  | 9.83  | 14.07 | 10.38 |
| 90              | 10.53 | 13.82                   | 20.44 | 9.84  | 11.03 | 9.90  | 8.46  | 9.86  | 10.85 |
| 100             | 12.93 | 15.30                   | 15.48 | 12.81 | 13.48 | 14.12 | 16.09 | 14.46 | 14.30 |
| 110             | 17.31 | 22.97                   | 18.00 | 17.03 | 17.96 | 20.67 | 18.73 | 20.66 | 16.85 |
| 120             | 21.91 | 19.93                   | 20.76 | 18.56 | 26.26 | 22.81 | 21.71 | 18.46 | 20.57 |
| 130             | 19.90 | 25.12                   | 22.47 | 34.23 | 20.59 | 28.69 | 33.91 | 24.01 | 21.09 |
| 140             | 22.75 | 35.67                   | 15.61 | 26.96 | 26.07 | 23.70 | 24.83 | 22.85 | 35.85 |

---

| Laser Power(mW) |       | Parts of Retardance(nm) |       |       |       |       |       |       |       |
|-----------------|-------|-------------------------|-------|-------|-------|-------|-------|-------|-------|
| 50              | 5.25  | 5.89                    | 4.80  | 4.83  | 5.07  | 4.74  | 4.76  | 4.37  | 4.35  |
| 60              | 4.89  | 5.65                    | 4.77  | 5.35  | 4.44  | 4.97  | 5.31  | 4.62  | 5.31  |
| 70              | 7.23  | 7.78                    | 6.40  | 6.79  | 7.18  | 7.24  | 6.76  | 7.19  | 7.22  |
| 80              | 9.66  | 9.44                    | 10.11 | 10.20 | 9.72  | 15.38 | 10.64 | 8.51  | 9.16  |
| 90              | 10.53 | 8.28                    | 9.51  | 9.17  | 8.48  | 9.76  | 10.53 | 8.70  | 9.16  |
| 100             | 14.70 | 12.85                   | 13.02 | 13.73 | 14.27 | 13.00 | 19.75 | 16.39 | 15.29 |
| 110             | 17.60 | 18.09                   | 20.68 | 17.03 | 21.67 | 21.85 | 18.83 | 20.10 | 16.59 |
| 120             | 23.27 | 22.11                   | 21.00 | 21.38 | 19.06 | 19.05 | 20.36 | 20.82 | 20.86 |
| 130             | 29.53 | 28.52                   | 30.59 | 33.49 | 29.15 | 21.50 | 20.16 | 24.53 | 18.88 |
| 140             | 30.89 | 15.87                   | 31.22 | 31.79 | 30.23 | 29.77 | 24.59 | 27.36 | 27.11 |

---

| Laser Power(mW) |       | Parts of Retardance(nm) |       |       |       |       |       |       |       |
|-----------------|-------|-------------------------|-------|-------|-------|-------|-------|-------|-------|
| 50              | 5.25  | 5.89                    | 4.80  | 4.83  | 5.07  | 4.74  | 4.76  | 4.37  | 4.35  |
| 60              | 4.89  | 5.65                    | 4.77  | 5.35  | 4.44  | 4.97  | 5.31  | 4.62  | 5.31  |
| 70              | 7.23  | 7.78                    | 6.40  | 6.79  | 7.18  | 7.24  | 6.76  | 7.19  | 7.22  |
| 80              | 9.66  | 9.44                    | 10.11 | 10.20 | 9.72  | 15.38 | 10.64 | 8.51  | 9.16  |
| 90              | 10.53 | 8.28                    | 9.51  | 9.17  | 8.48  | 9.76  | 10.53 | 8.70  | 9.16  |
| 100             | 14.70 | 12.85                   | 13.02 | 13.73 | 14.27 | 13.00 | 19.75 | 16.39 | 15.29 |
| 110             | 17.60 | 18.09                   | 20.68 | 17.03 | 21.67 | 21.85 | 18.83 | 20.10 | 16.59 |
| 120             | 23.27 | 22.11                   | 21.00 | 21.38 | 19.06 | 19.05 | 20.36 | 20.82 | 20.86 |
| 130             | 29.53 | 28.52                   | 30.59 | 33.49 | 29.15 | 21.50 | 20.16 | 24.53 | 18.88 |
| 140             | 30.89 | 15.87                   | 31.22 | 31.79 | 30.23 | 29.77 | 24.59 | 27.36 | 27.11 |

Table 2: The relationship between pulse number and retardance(0 degree).

| Pulse number |       | Parts of Retardance(nm) |       |       |       |       |       |       |       |
|--------------|-------|-------------------------|-------|-------|-------|-------|-------|-------|-------|
| 50           | 4.11  | 4.29                    | 4.96  | 5.48  | 4.53  | 4.63  | 4.78  | 5.79  | 4.62  |
| 60           | 5.12  | 6.40                    | 6.17  | 5.99  | 6.37  | 5.78  | 5.84  | 5.75  | 5.78  |
| 70           | 6.66  | 6.74                    | 7.38  | 7.23  | 7.68  | 7.70  | 8.04  | 9.16  | 8.05  |
| 80           | 12.21 | 10.66                   | 9.99  | 10.51 | 10.67 | 9.84  | 9.74  | 12.80 | 8.17  |
| 90           | 10.85 | 10.53                   | 10.44 | 11.03 | 11.69 | 12.86 | 13.96 | 12.53 | 9.46  |
| 100          | 10.52 | 13.99                   | 14.30 | 16.52 | 20.27 | 17.60 | 14.12 | 16.09 | 18.16 |
| 110          | 18.22 | 17.11                   | 20.12 | 18.20 | 16.90 | 22.74 | 16.51 | 18.36 | 18.69 |
| 120          | 21.05 | 20.02                   | 19.11 | 18.17 | 19.92 | 27.62 | 19.80 | 20.21 | 21.69 |
| 130          | 23.51 | 20.77                   | 20.47 | 26.18 | 20.63 | 22.41 | 25.44 | 21.06 | 22.80 |
| 140          | 24.57 | 23.60                   | 27.57 | 26.59 | 25.93 | 23.68 | 26.06 | 24.08 | 24.43 |

Table 3: The relationship between pulse number and retardance(30 degree).

| Pulse number | Parts of Retardance(nm) |       |       |       |       |      |       |       |       |
|--------------|-------------------------|-------|-------|-------|-------|------|-------|-------|-------|
| 200          | 6.09                    | 6.46  | 6.84  | 6.07  | 7.63  | 6.85 | 6.44  | 6.58  | 6.8   |
| 400          | 6.87                    | 7.02  | 6.84  | 6.41  | 7.46  | 6.4  | 5.49  | 7.16  | 8.43  |
| 600          | 6.77                    | 6.55  | 8.16  | 5.67  | 8.64  | 7.88 | 7.46  | 6.07  | 7.04  |
| 800          | 6.87                    | 6.59  | 7.61  | 8.22  | 8.72  | 7.92 | 6.72  | 6.79  | 8.7   |
| 1000         | 8.54                    | 9.04  | 11    | 8.58  | 9.17  | 7.89 | 7.81  | 9.81  | 11.61 |
| 1200         | 8.1                     | 8.37  | 8.55  | 6.27  | 9.04  | 8.26 | 6.78  | 7.99  | 7.99  |
| 1400         | 9.15                    | 9.42  | 7.08  | 9.44  | 8.6   | 6.99 | 7.53  | 8.34  | 9.58  |
| 1600         | 10.94                   | 11.26 | 8.45  | 11.29 | 10.28 | 8.35 | 9     | 9.97  | 11.45 |
| 1800         | 10.07                   | 10.38 | 7.73  | 10.41 | 9.45  | 7.63 | 8.24  | 9.16  | 10.56 |
| 2000         | 10.73                   | 10.56 | 10.43 | 12.18 | 10.58 | 9.9  | 11.55 | 11.01 | 12.27 |

Table 4: The relationship between pulse number and retardance(60 degree).

| Pulse number | Parts of Retardance(nm) |       |       |       |       |       |       |       |       |
|--------------|-------------------------|-------|-------|-------|-------|-------|-------|-------|-------|
| 200          | 7.02                    | 7.11  | 6.32  | 7.12  | 6.83  | 6.29  | 6.48  | 6.75  | 7.16  |
| 400          | 7.51                    | 7.65  | 6.4   | 7.67  | 7.21  | 6.35  | 6.64  | 7.08  | 7.74  |
| 600          | 7.69                    | 7.12  | 7.12  | 7.81  | 7.19  | 7.58  | 7.28  | 7.5   | 8     |
| 800          | 7.86                    | 8.61  | 8.86  | 7.04  | 8.9   | 7.9   | 7.51  | 8.97  | 8.13  |
| 1000         | 9.04                    | 9.43  | 10.1  | 10.2  | 10.32 | 9.96  | 10.36 | 10.73 | 9.24  |
| 1200         | 9.88                    | 10.16 | 9.44  | 10.3  | 9.24  | 10.7  | 10.32 | 9.31  | 9.94  |
| 1400         | 8.29                    | 8.89  | 8.01  | 8.35  | 8.89  | 7.62  | 7.44  | 8.2   | 8.52  |
| 1600         | 10.9                    | 9.73  | 10.46 | 10.82 | 11.33 | 11.03 | 10.47 | 11.58 | 10.08 |
| 1800         | 10.36                   | 9.59  | 8.88  | 9.88  | 8.59  | 9.66  | 8.66  | 9.2   | 10.39 |
| 2000         | 10.32                   | 10.65 | 12.21 | 10.43 | 9.86  | 11.88 | 10.95 | 12.28 | 11.69 |

## 4 Trade-off between storage information capacity and redundancy length.

Through our investigation, we have observed that as the layer spacing decreases while maintaining a fixed point spacing, the data accuracy also decreases. This prompted us to explore the optimal voxel layer spacing for preserving data accuracy as shown in Table 5. Subsequently, we conducted a comprehensive test, wherein we systematically reduced the point spacing under the identified preferred layer spacing of 10 microns. The findings of this test are presented in Table 6, illustrating the impact on data accuracy at varying point spacing. To enhance data encoding capacity, we employed different bit numbers for data encoding, focusing on improving color distinction and size distinction. The outcomes of this encoding strategy are outlined in Table 7, showcasing the achieved data encoding capacities with varying bit numbers. Take a similar approach as before, we employed the TPH-YOLOv5 algorithm for precise data localization, and the VGG16 algorithm for data classification in order to accurately locate and classify the data.

Table 5: The relationship between accuracy, redundancy length and layer spacing. (Point spacing:  $3 \mu m$ , number of codes: 5 bits)

| Layer spacing( $\mu m$ ) | Accuracy(%) | Redundancy length (bits) |
|--------------------------|-------------|--------------------------|
| 15                       | 97.48       | 13                       |
| 12                       | 97.53       | 13                       |
| 10                       | 98.68       | 8                        |
| 9                        | 91.03       | 46                       |
| 8                        | 81.86       | 97                       |

Table 6: The relationship between accuracy, redundancy length and point spacing. (Layer spacing: 10  $\mu m$ , number of codes: 5 bits)

| Point spacing( $\mu m$ ) | Accuracy(%) | Redundancy length (bits) |
|--------------------------|-------------|--------------------------|
| 3                        | 93.21       | 36                       |
| 2                        | 92.18       | 41                       |
| 1.5                      | 92.92       | 41                       |
| 1.4                      | 70.19       | 153                      |
| 1.3                      | 70.20       | 153                      |

Table 7: The relationship between accuracy, redundancy length, capacity, ratio of real data capacity, real data capacity and number of codes. (Point spacing: 3  $\mu m$ , layer spacing: 10  $\mu m$ )

| Codes Num(bits) | Acc (%) | Redundancy (bits) | Capacity(Tb) | Ratio | Available Capacity(Tb) |
|-----------------|---------|-------------------|--------------|-------|------------------------|
| 4               | 99.88   | 5                 | 1.08         | 98    | 1.06                   |
| 5               | 98.50   | 8                 | 1.34         | 97    | 1.30                   |
| 6               | 97.54   | 13                | 1.61         | 95    | 1.53                   |
| 7               | 95.85   | 23                | 1.88         | 91    | 1.71                   |
| 8               | 92.50   | 38                | 2.15         | 85    | 1.83                   |

## 5 Display of data classification effects.

We use a confusion matrix to compare real data and predicted values. The horizontal axis is predicted data, and the vertical axis is measured data. We cross-checked each group using more than 300 points of data to determine its identification mechanism. It can be seen that based on a large amount of data, there will be data recognition errors, which illustrates the necessity of adding error correction codes.

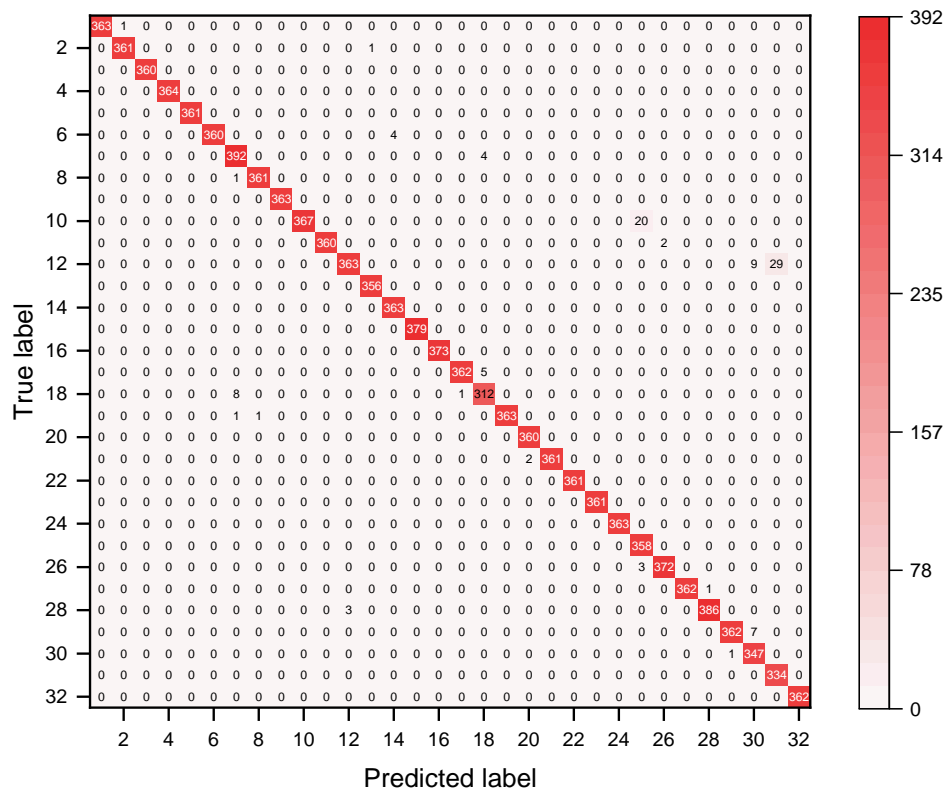

Figure 7:  $32 \times 32$  classification confusion matrix (16 categories for slow axis azimuth and 2 categories for retardance).

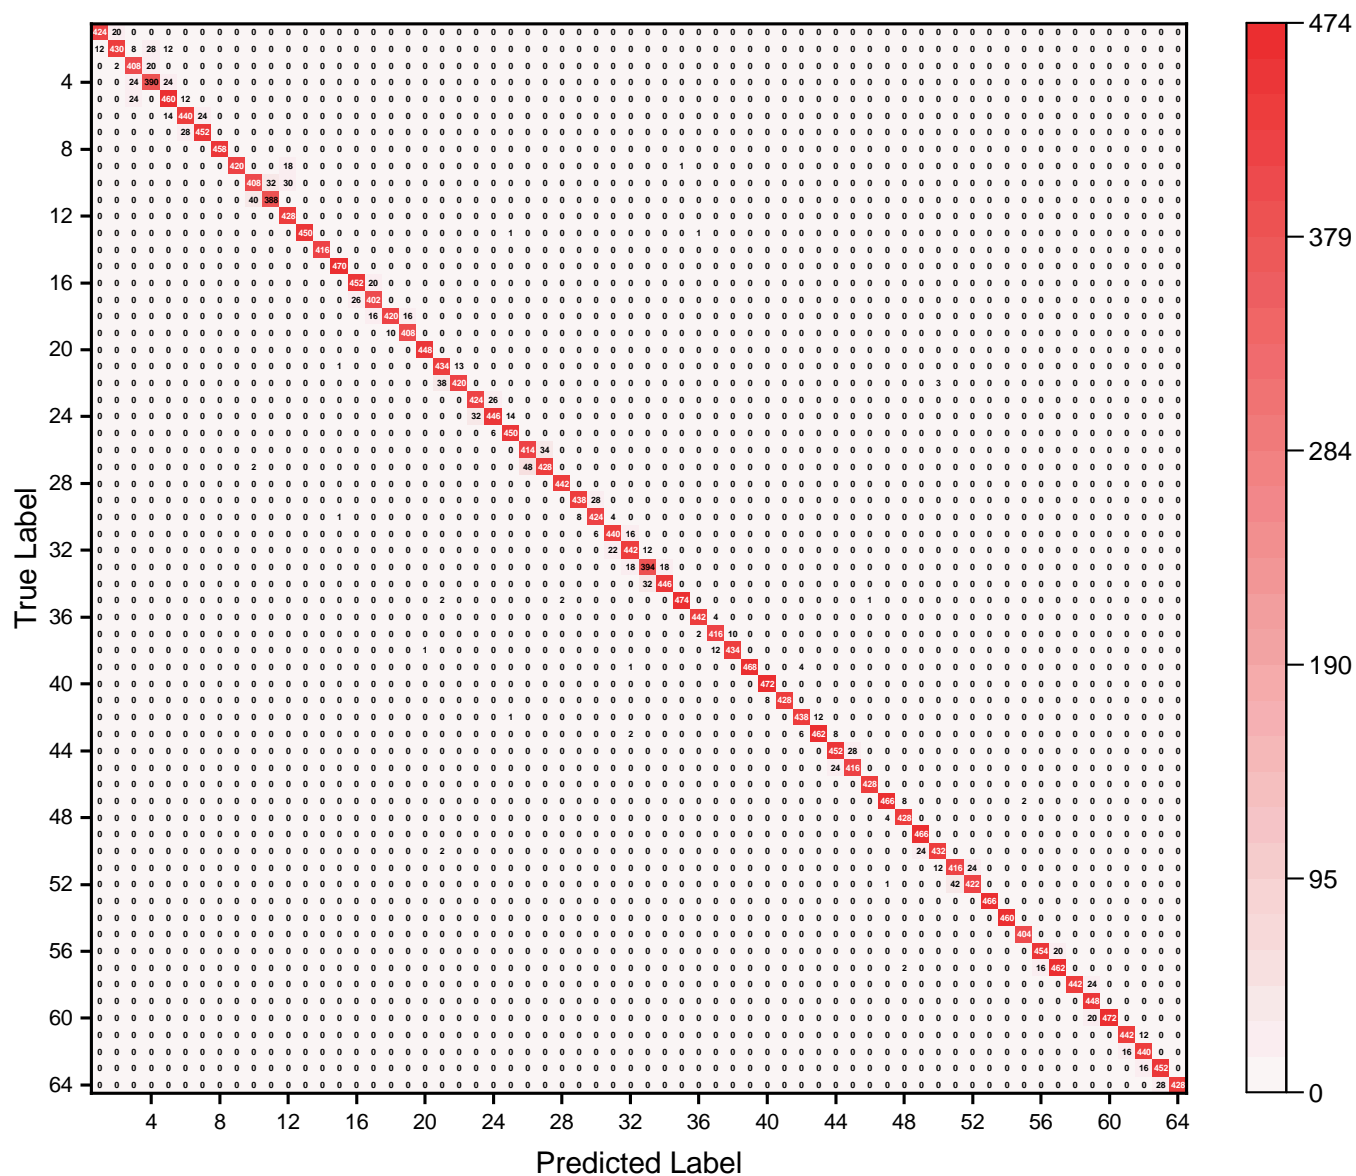

Figure 8:  $64 \times 64$  classification confusion matrix (16 categories for slow axis azimuth and 4 categories for retardance).

## 6 Display of label maps for 256 categories.

The following figure is based on 256 size classifications of 64 slow axis azimuth angles and 4 types of retardance. Among them, each square matrix in Figure 9-11(Part 1-3), Figure 12-14(Part 4-6), Figure 15-17(Part 7-9) and Figure 18-20(Part 10-12) represents 64 colors, and the corresponding labels have the same retardance.

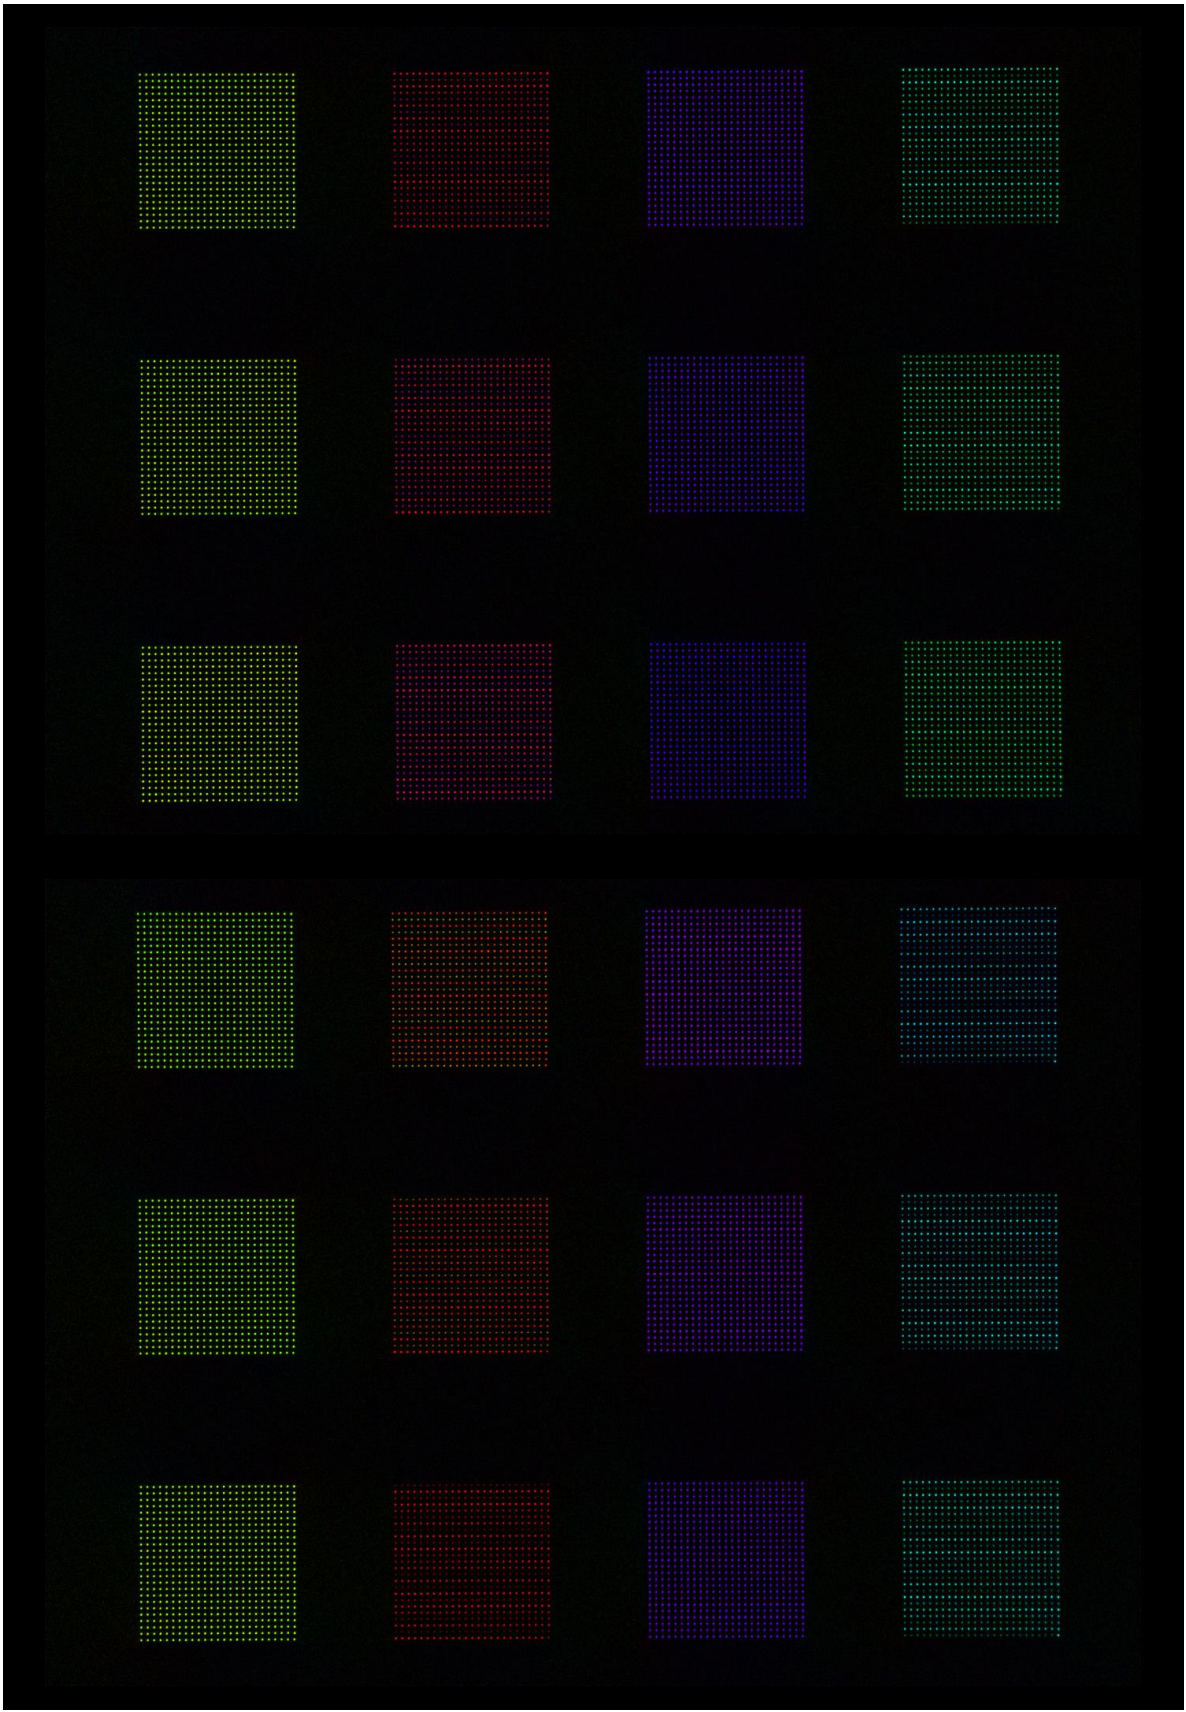

Figure 9: 8-bit dataset for encoded data of 256 classifications (Part 1).

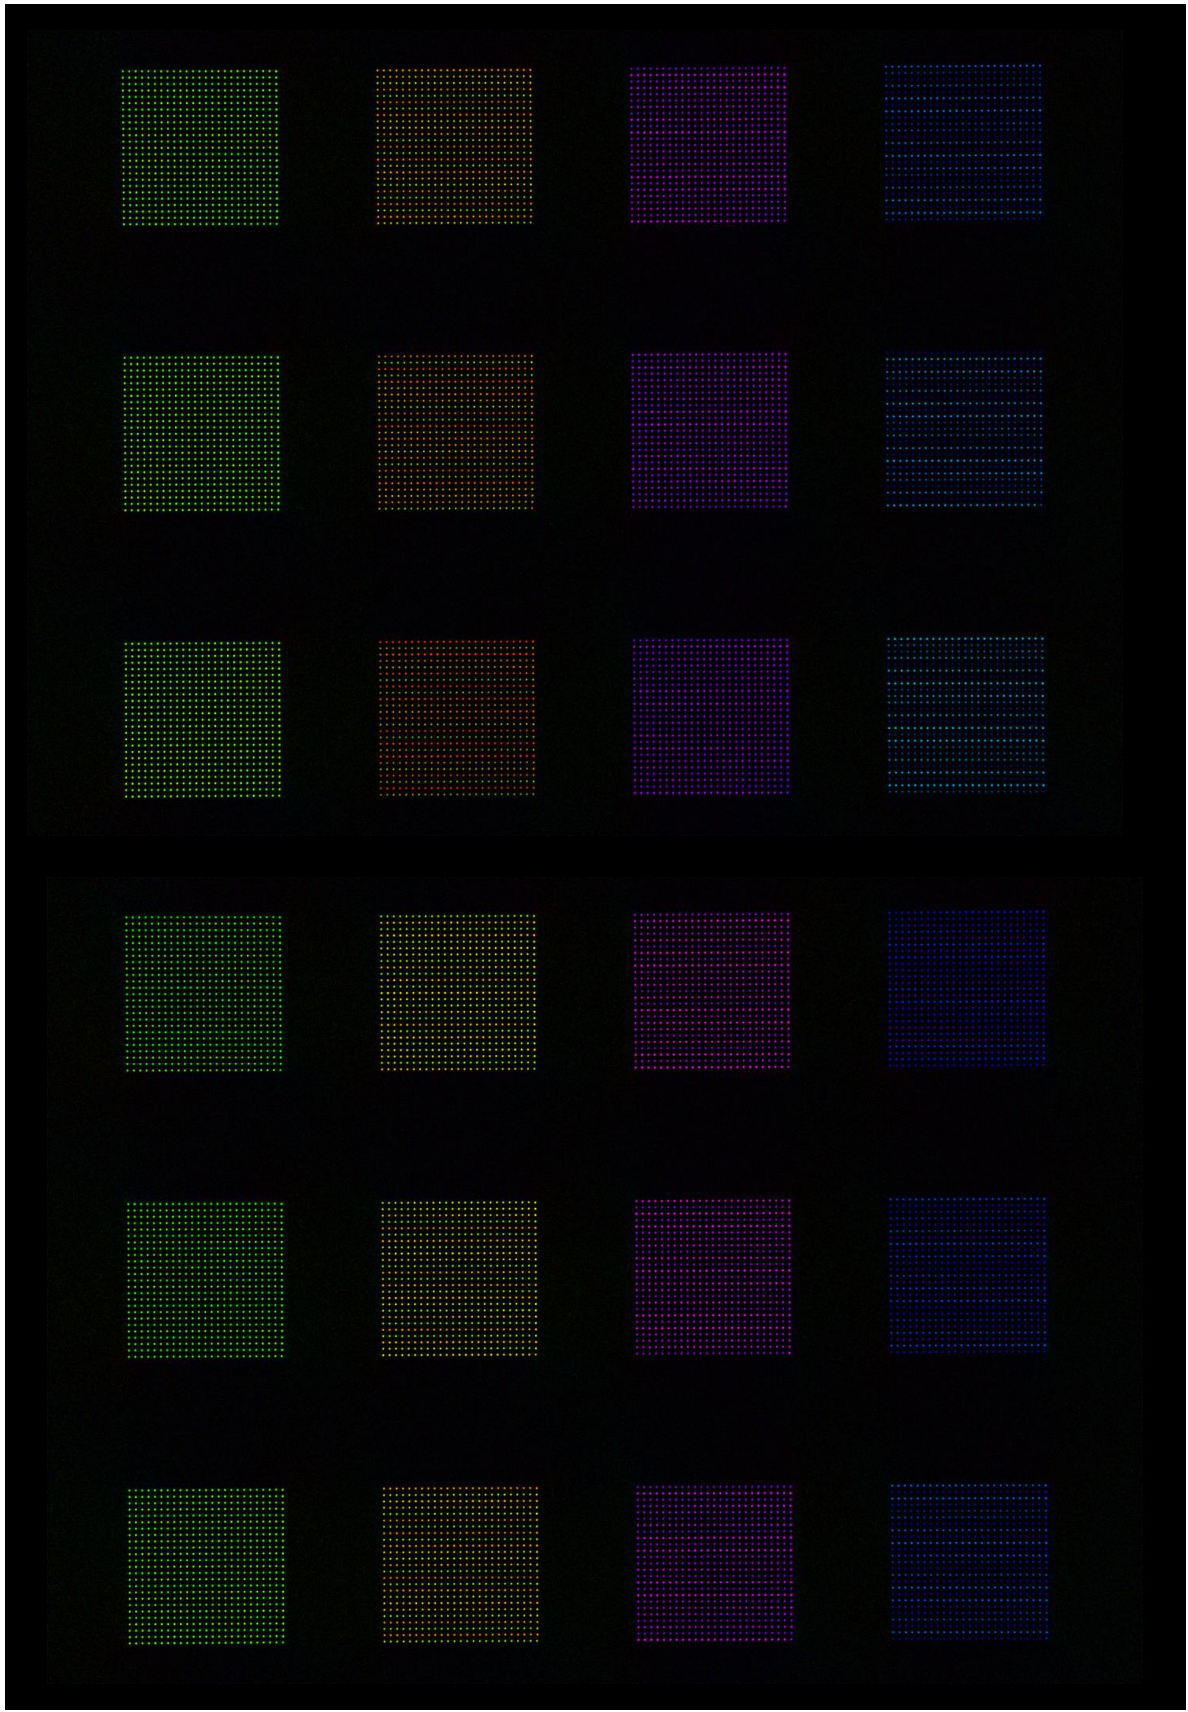

Figure 10: 8-bit dataset for encoded data of 256 classifications (Part 2).

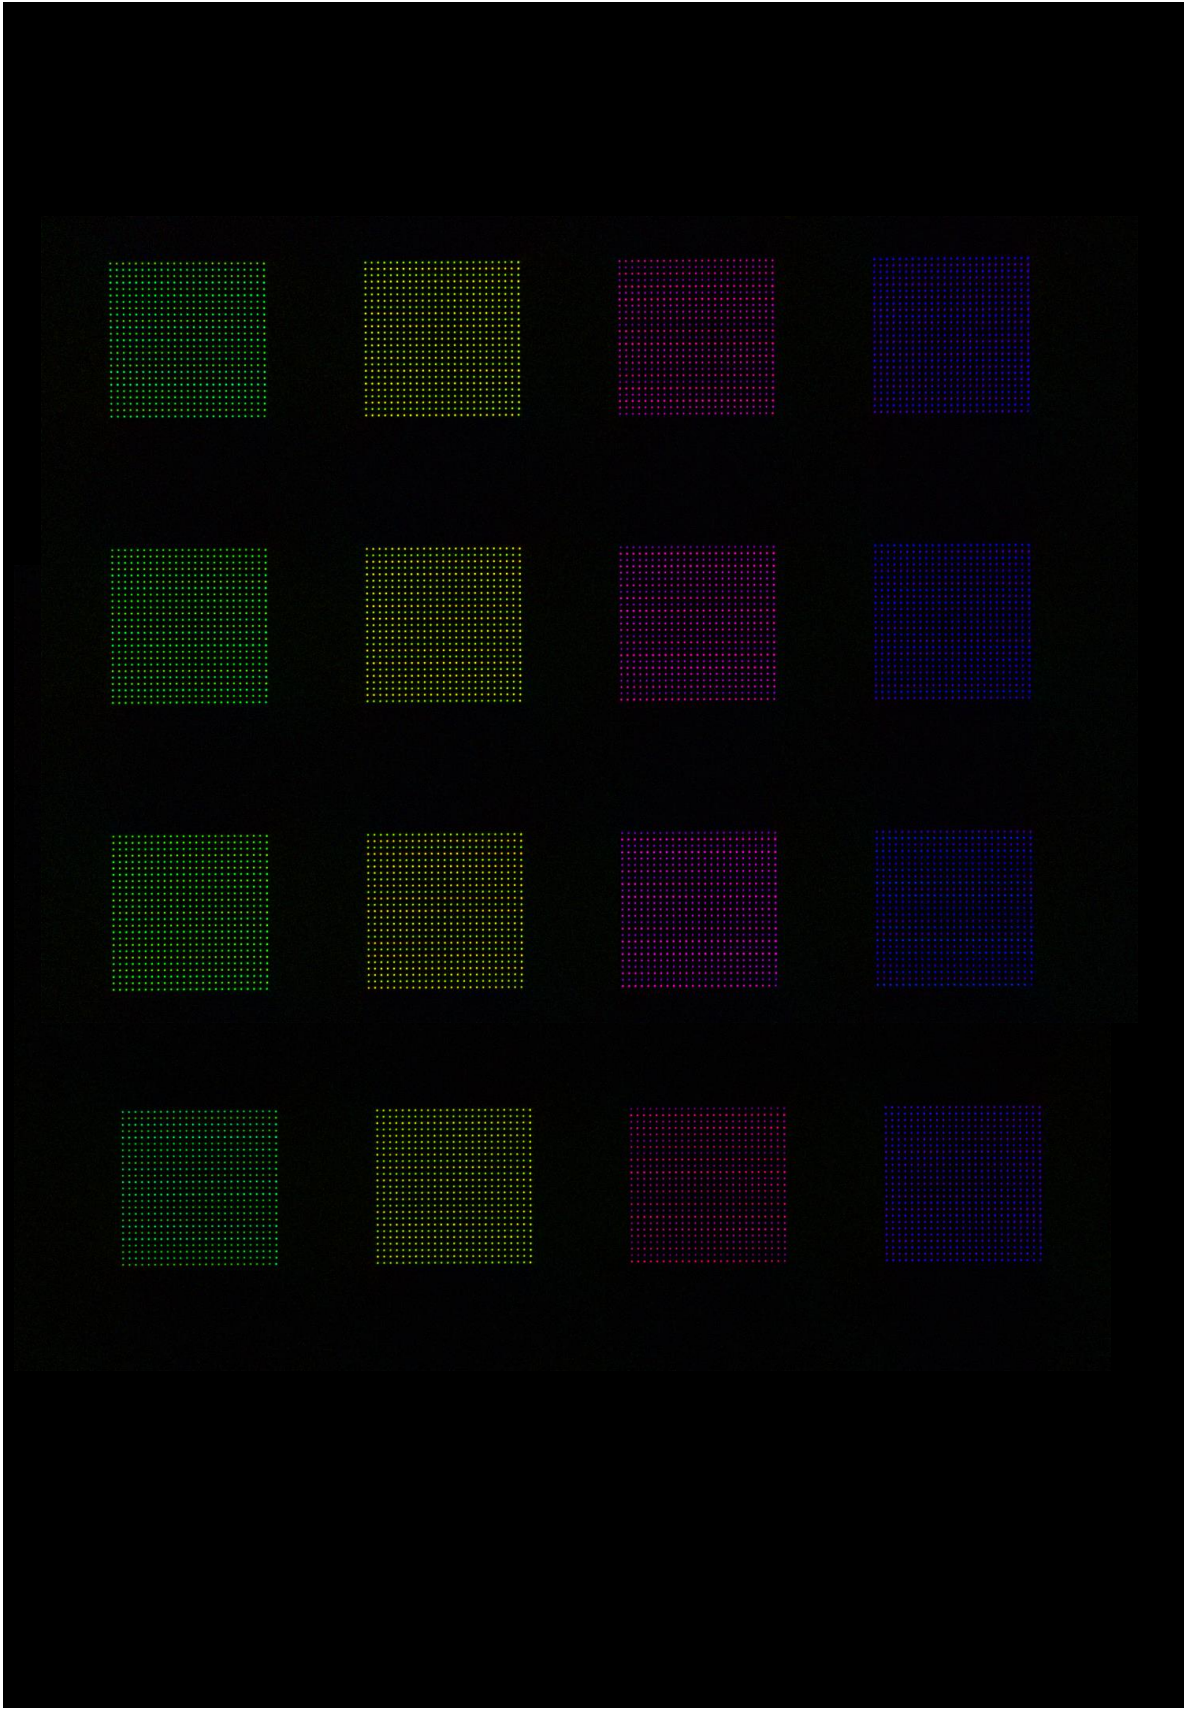

Figure 11: 8-bit dataset for encoded data of 256 classifications (Part 3).

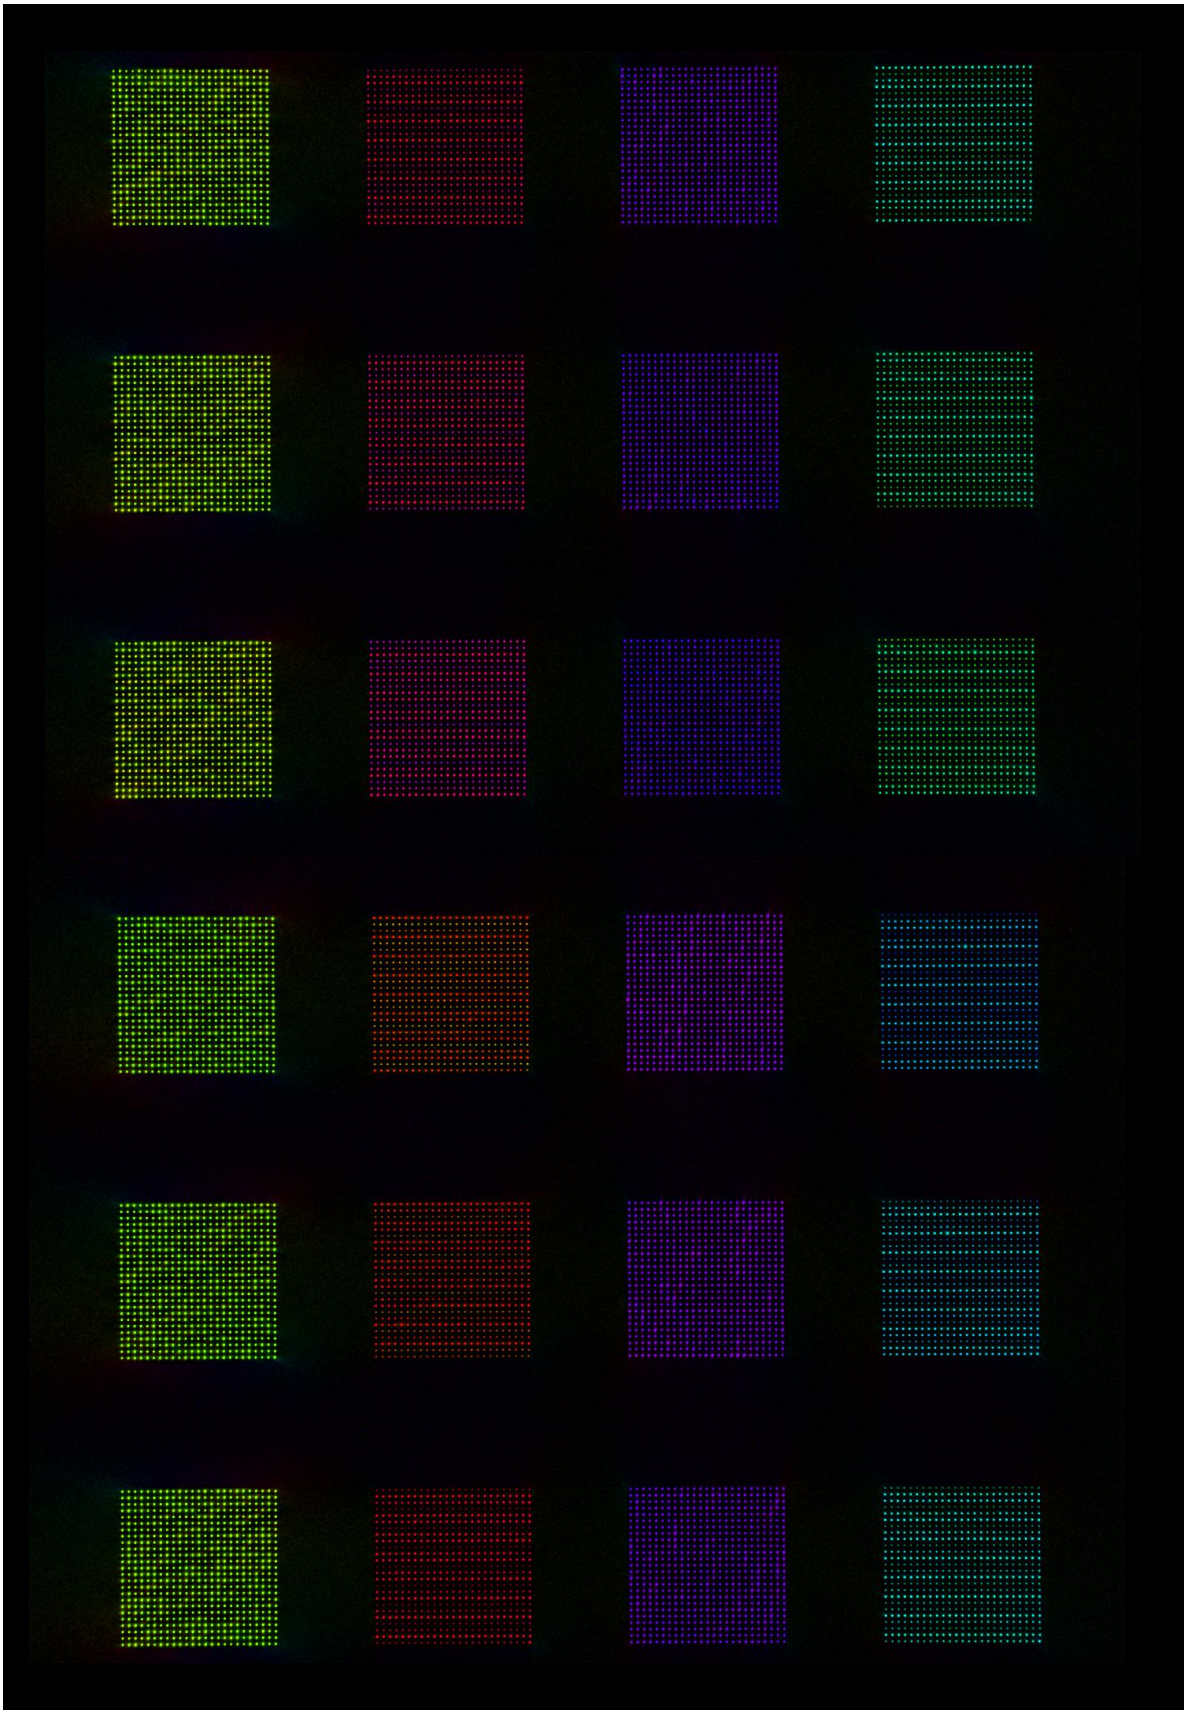

Figure 12: 8-bit dataset for encoded data of 256 classifications (Part 4).

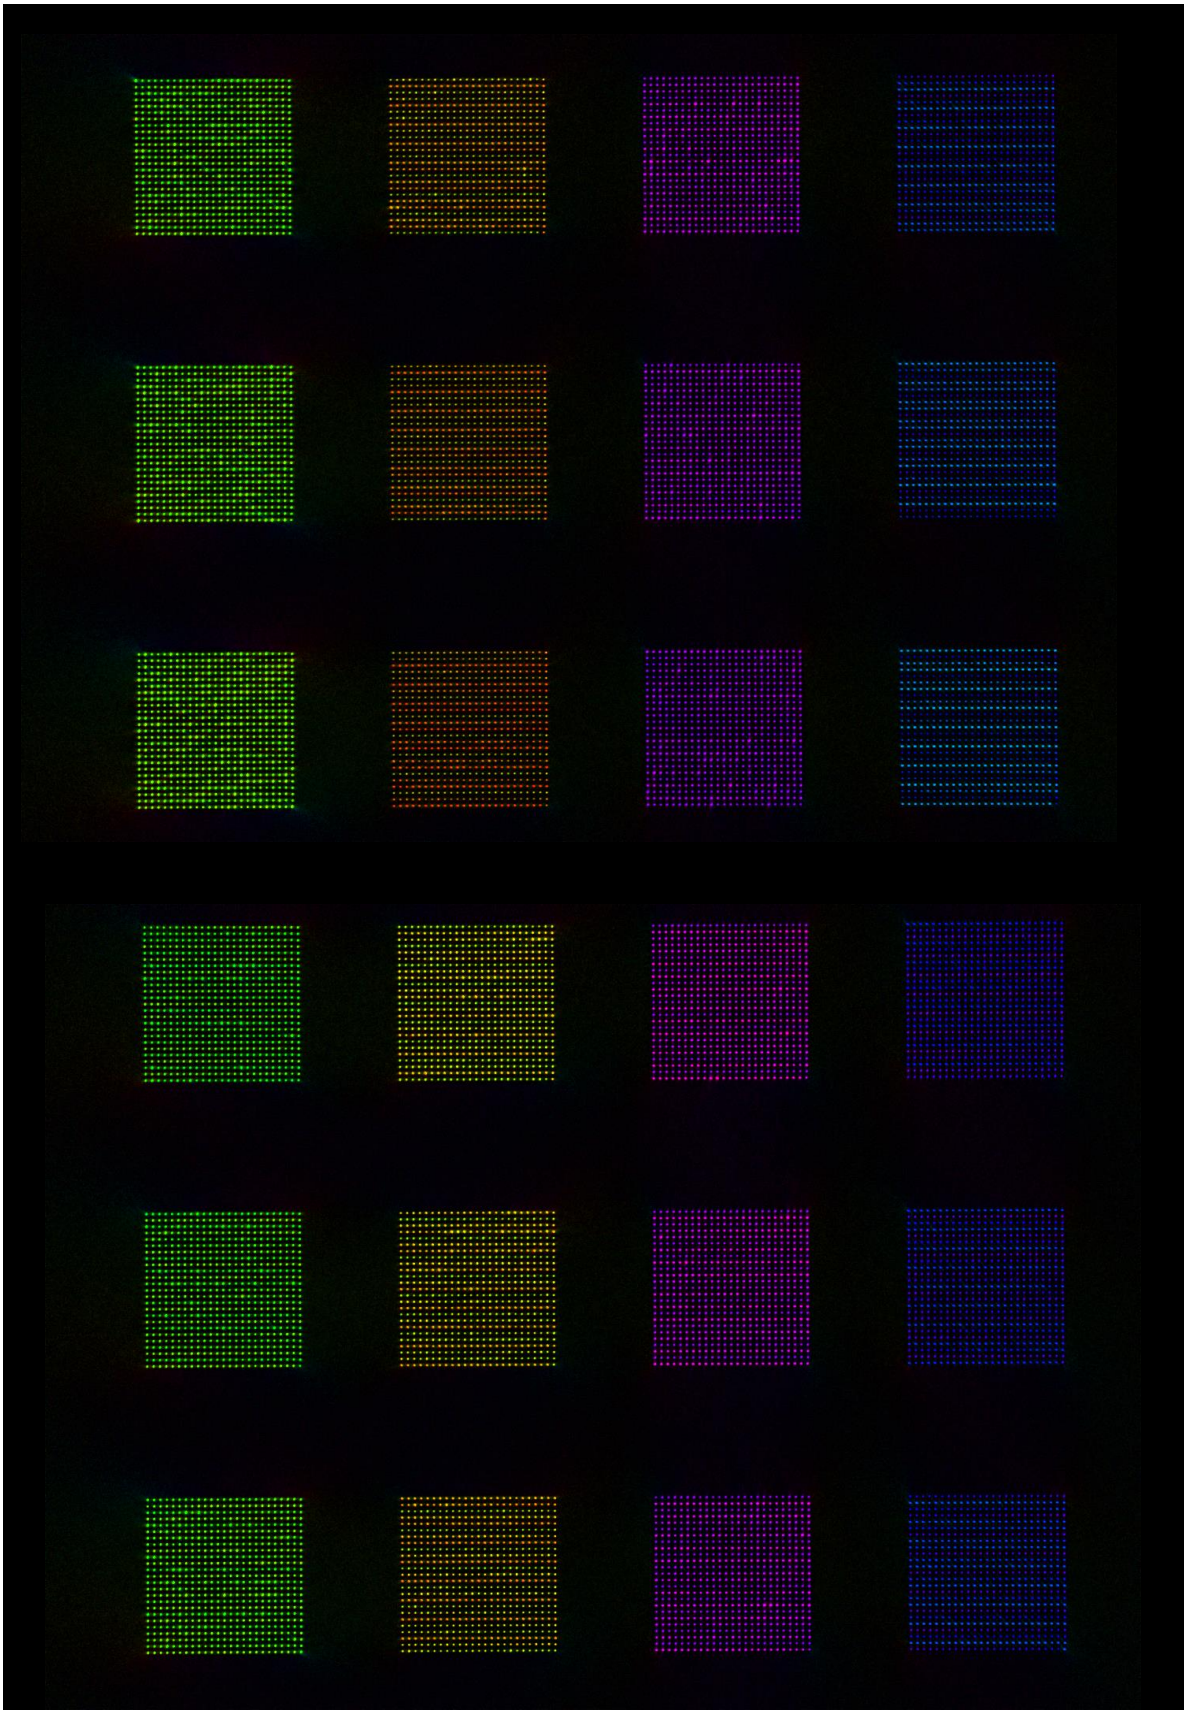

Figure 13: 8-bit dataset for encoded data of 256 classifications (Part 5).

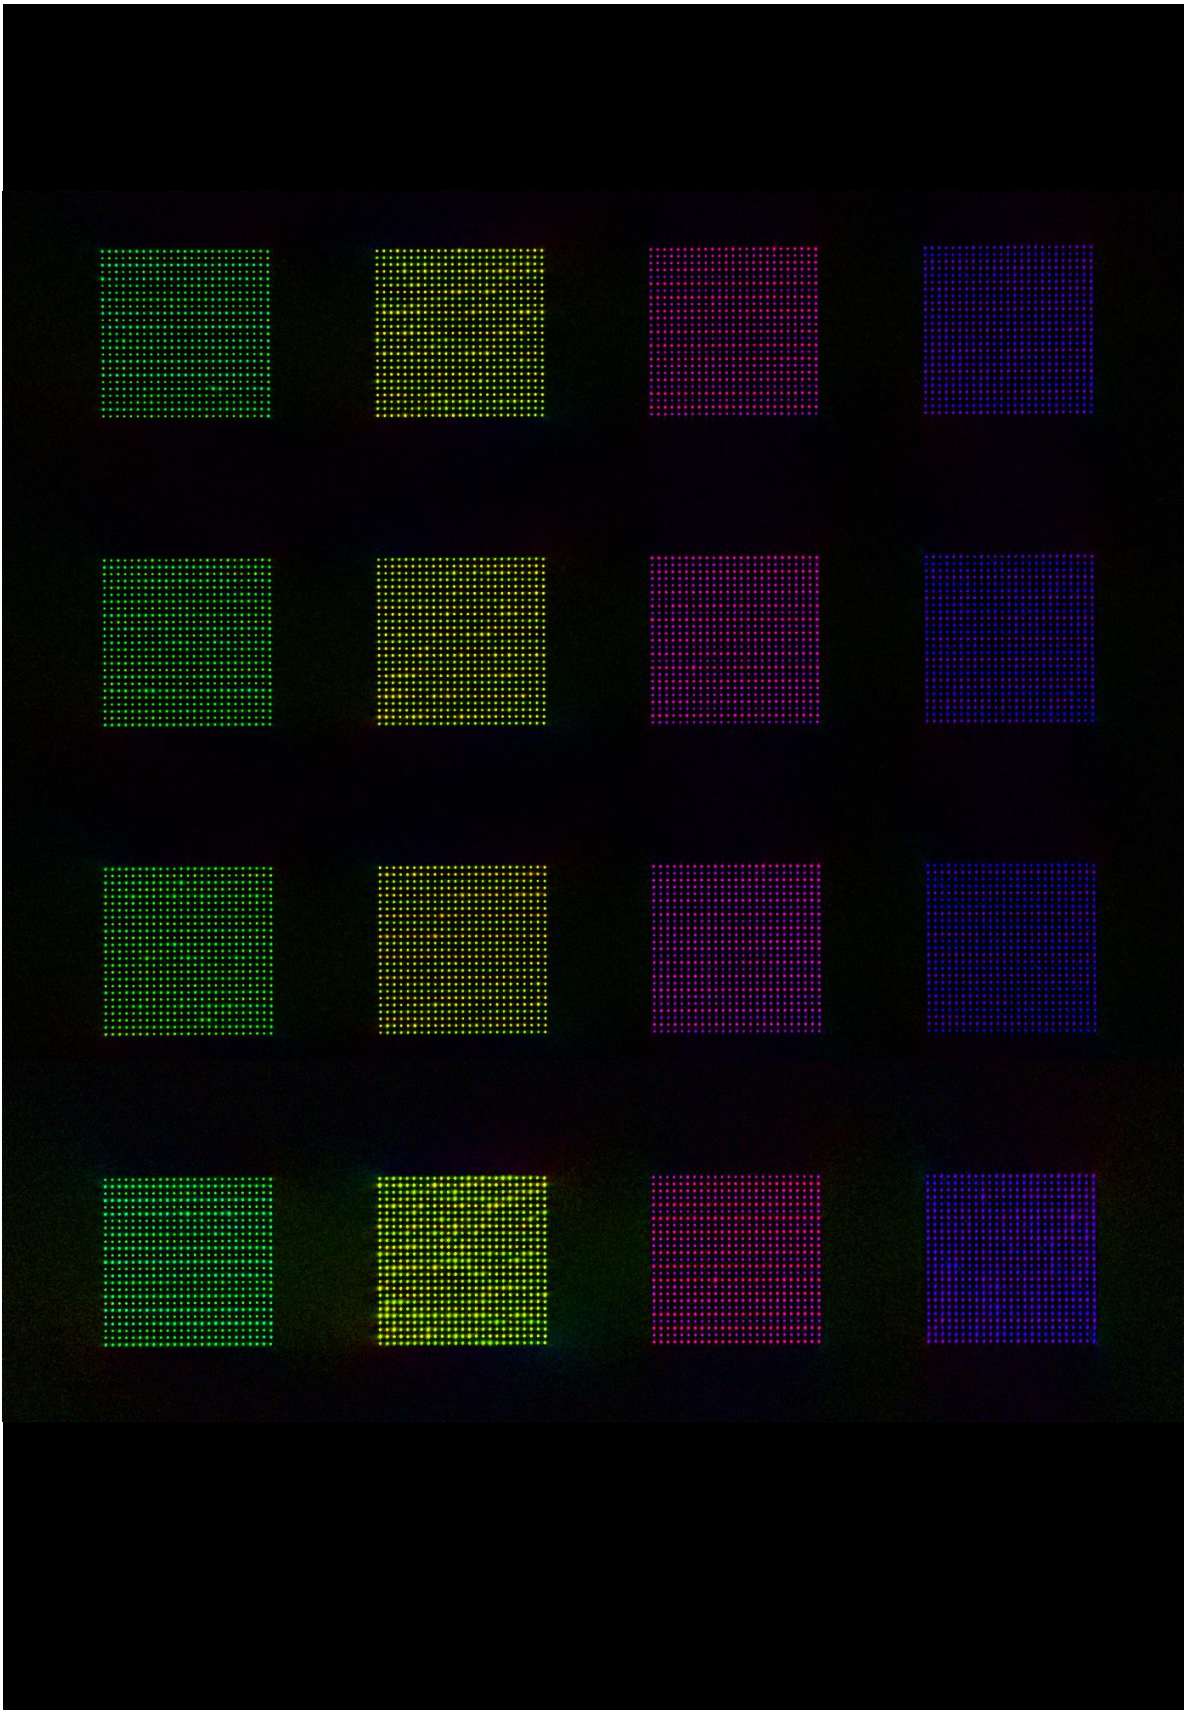

Figure 14: 8-bit dataset for encoded data of 256 classifications (Part 6).

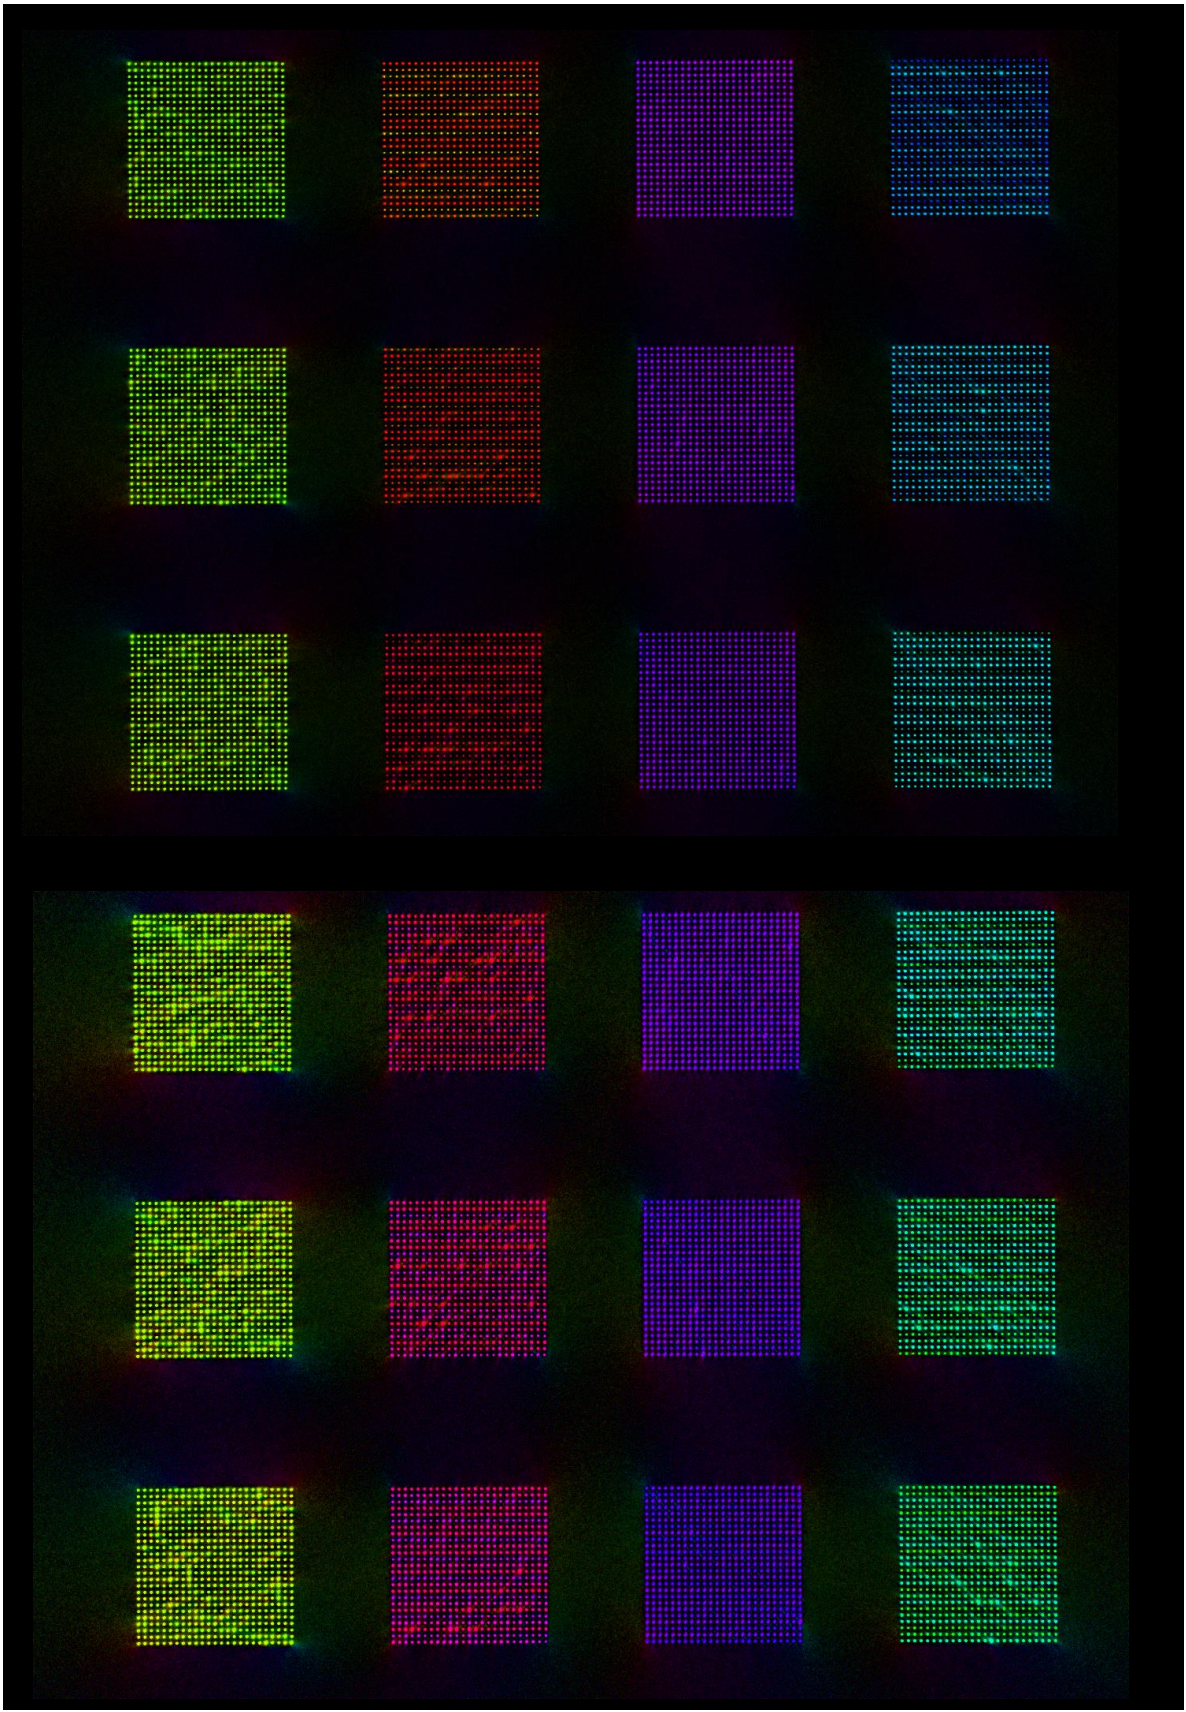

Figure 15: 8-bit dataset for encoded data of 256 classifications (Part 7).

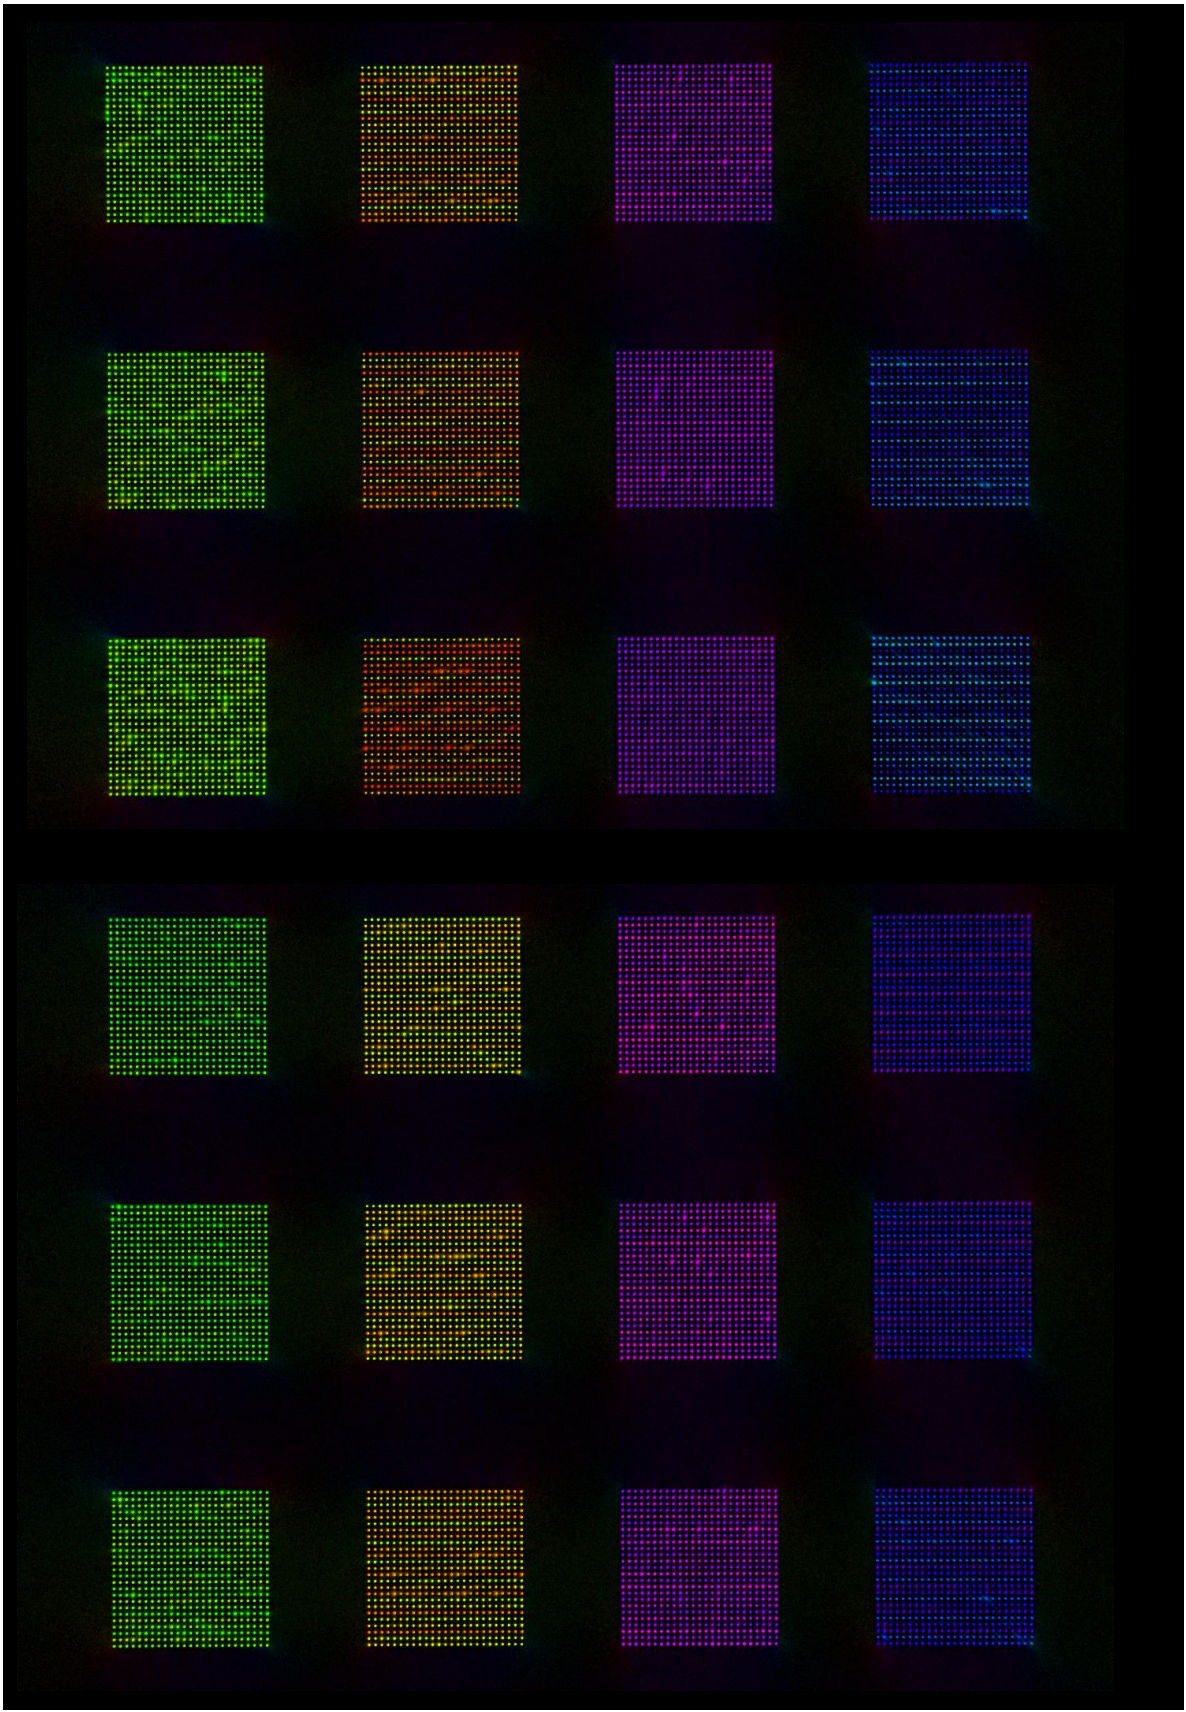

Figure 16: 8-bit dataset for encoded data of 256 classifications (Part 8).

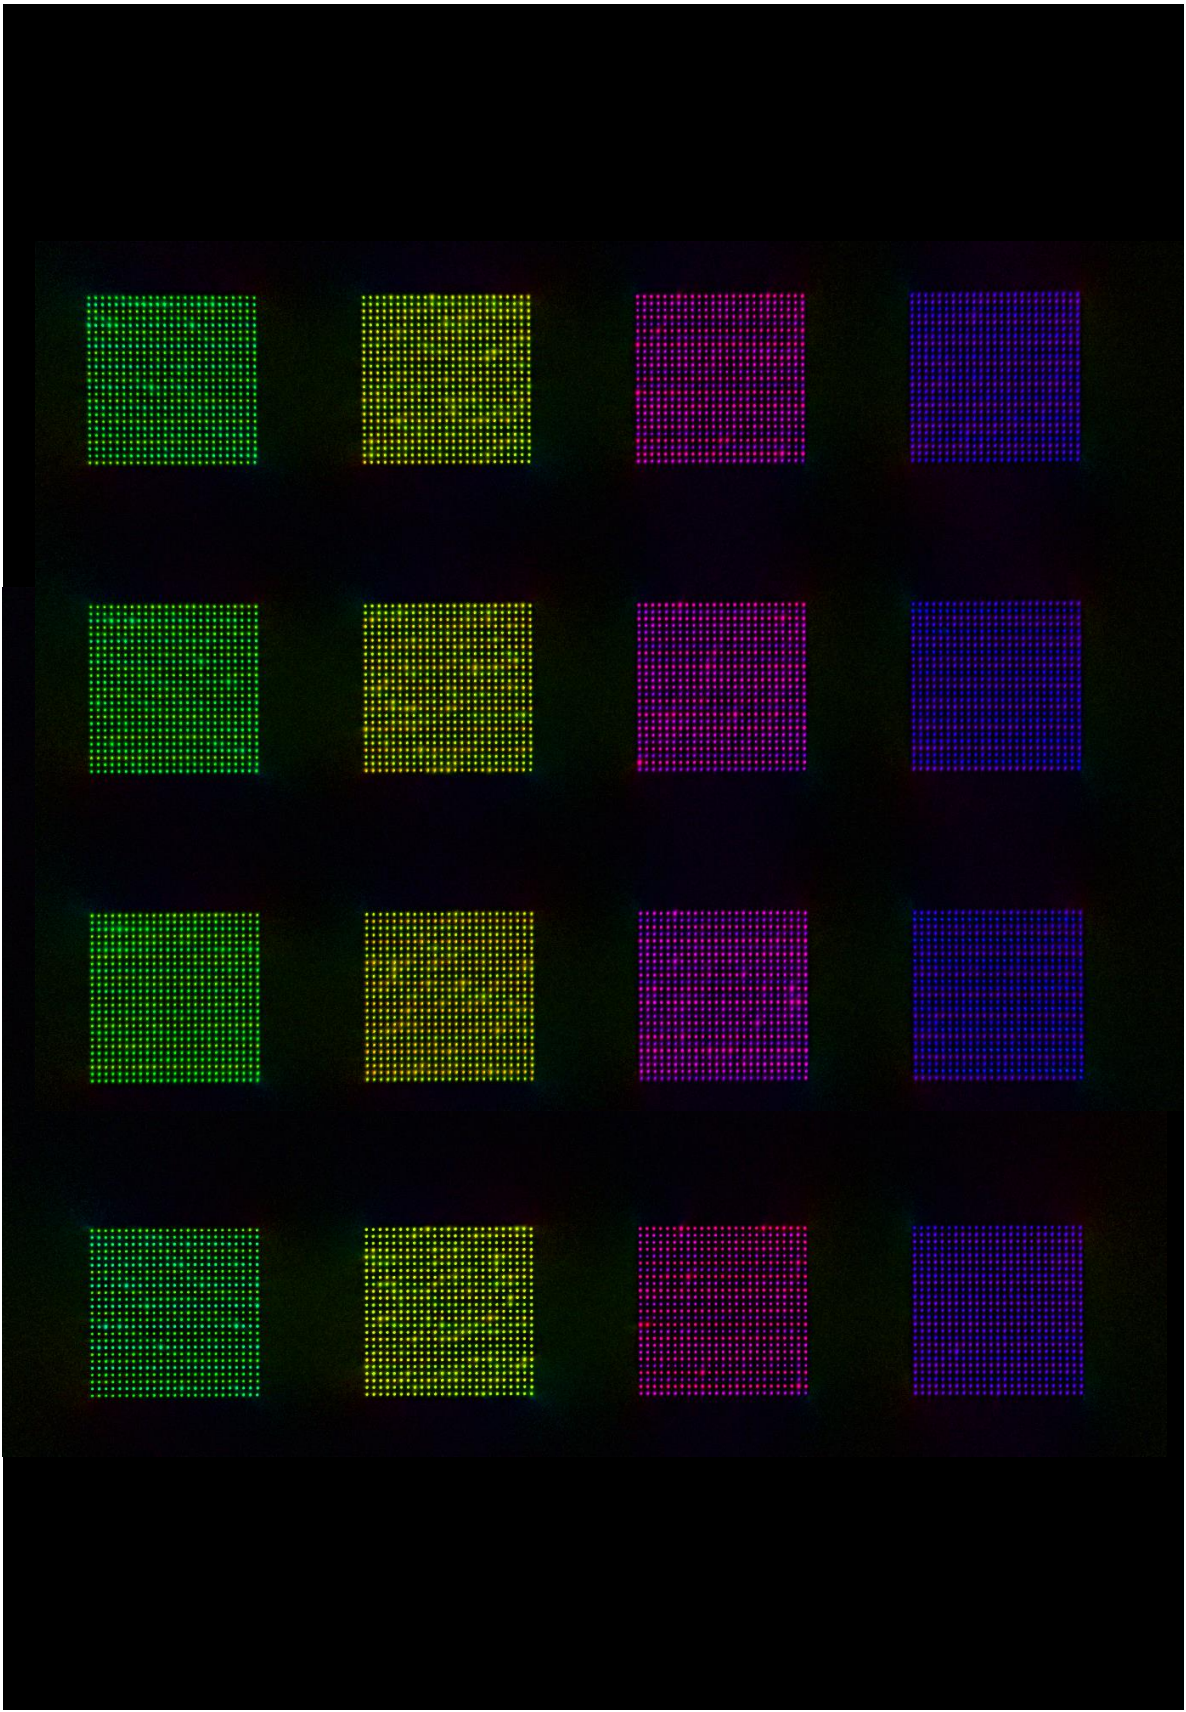

Figure 17: 8-bit dataset for encoded data of 256 classifications (Part 9).

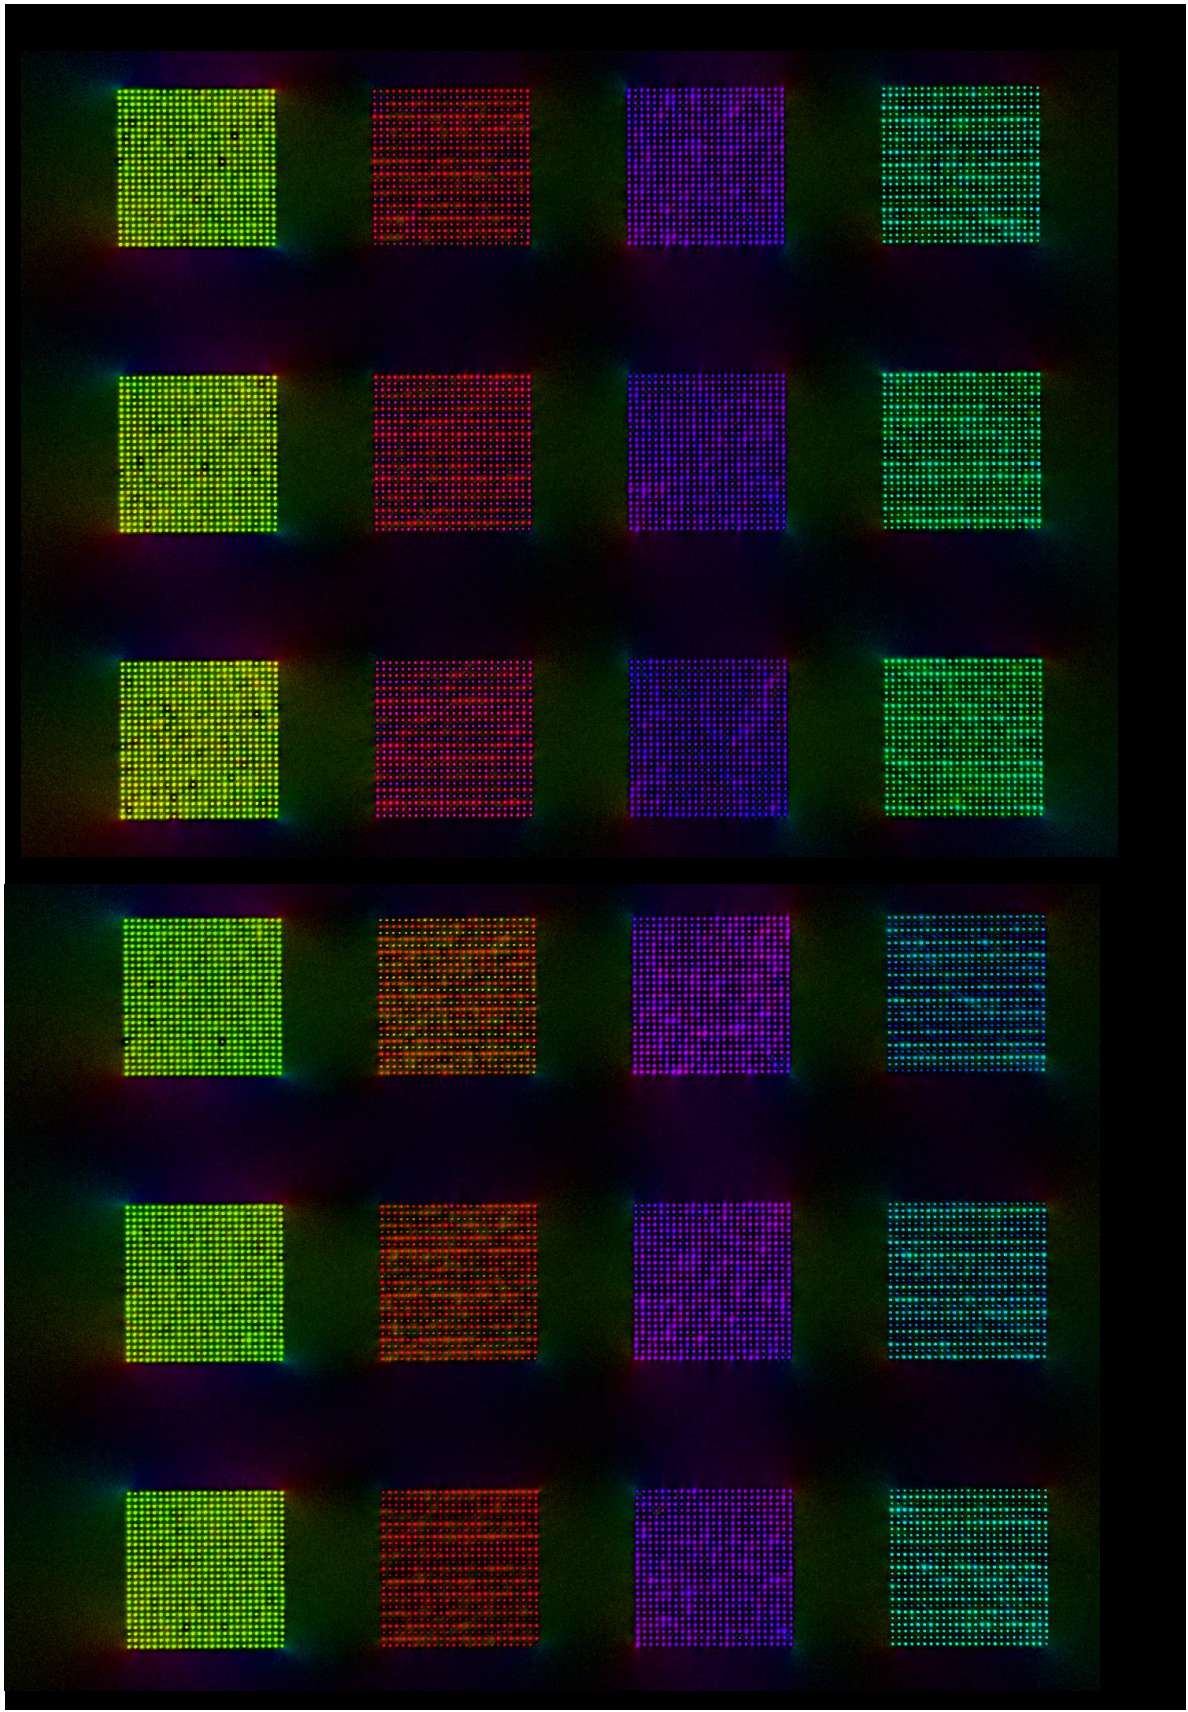

Figure 18: 8-bit dataset for encoded data of 256 classifications (Part 10).

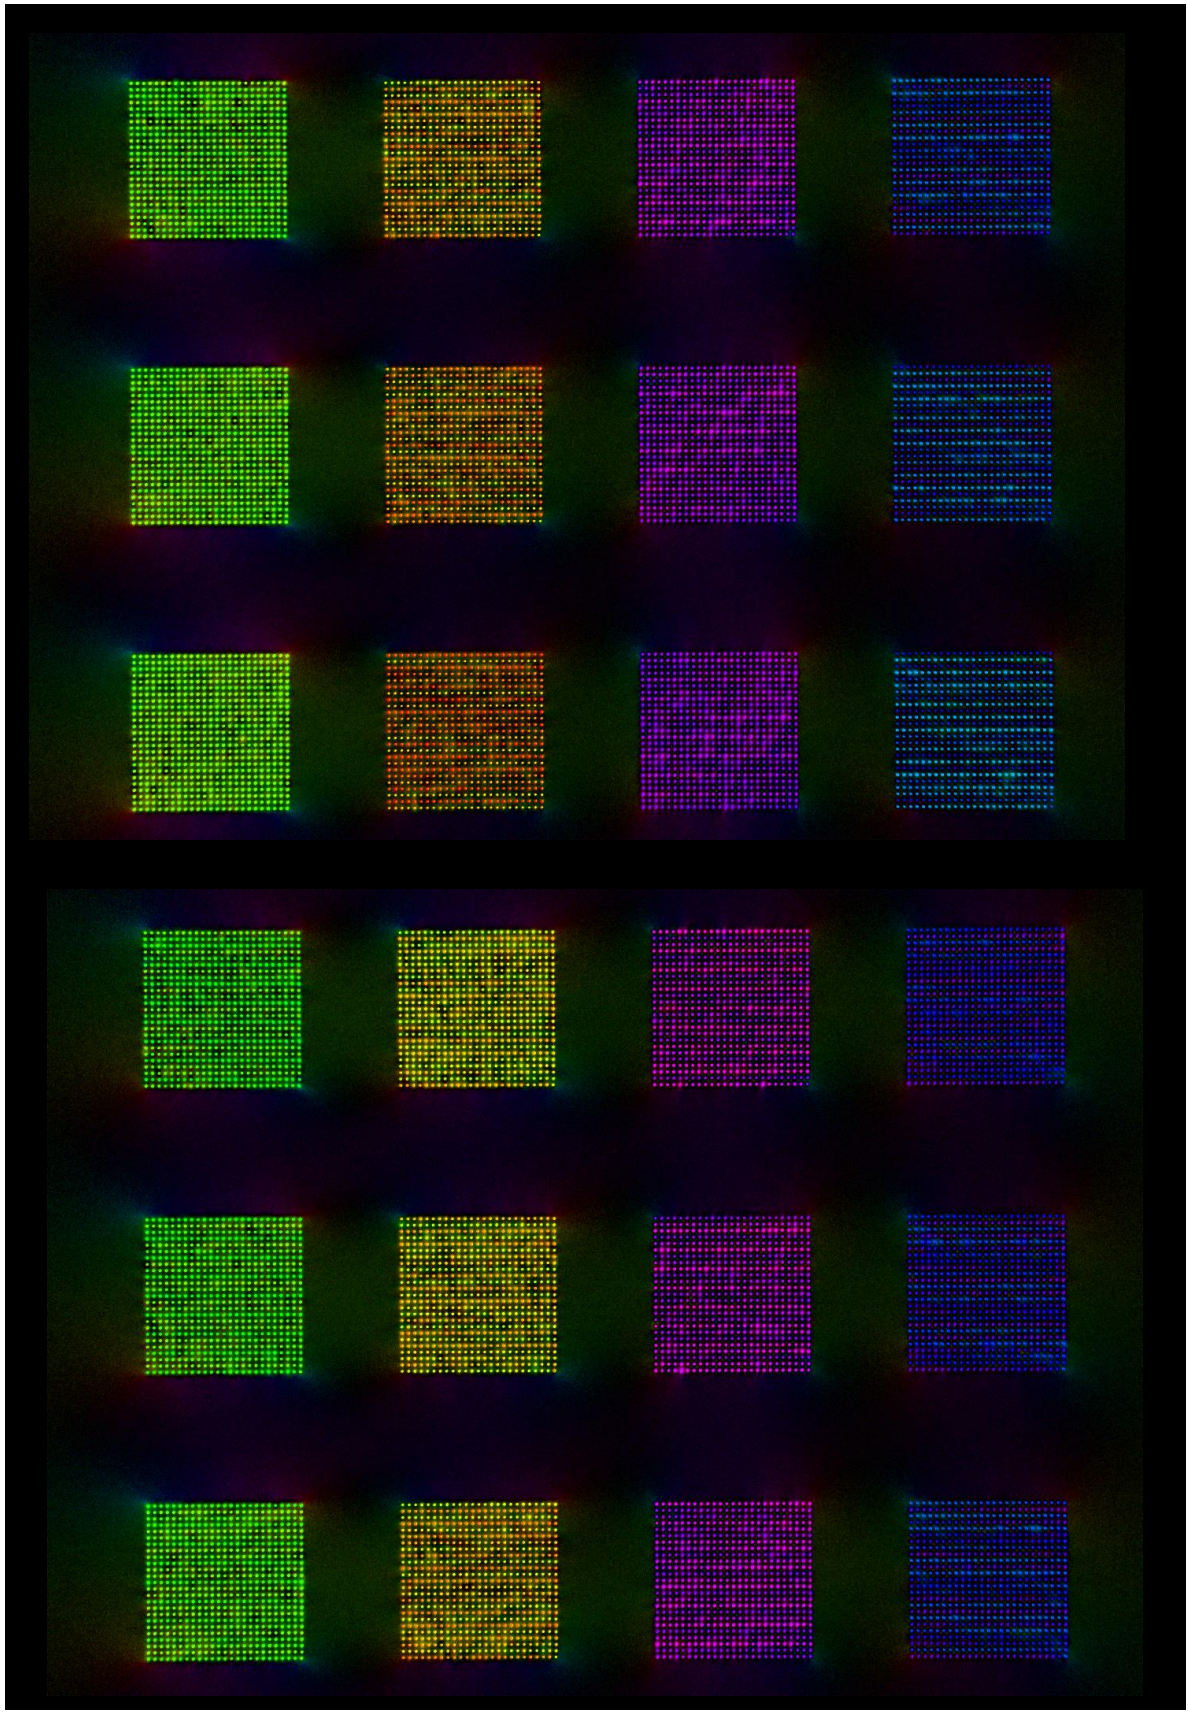

Figure 19: 8-bit dataset for encoded data of 256 classifications (Part 11).

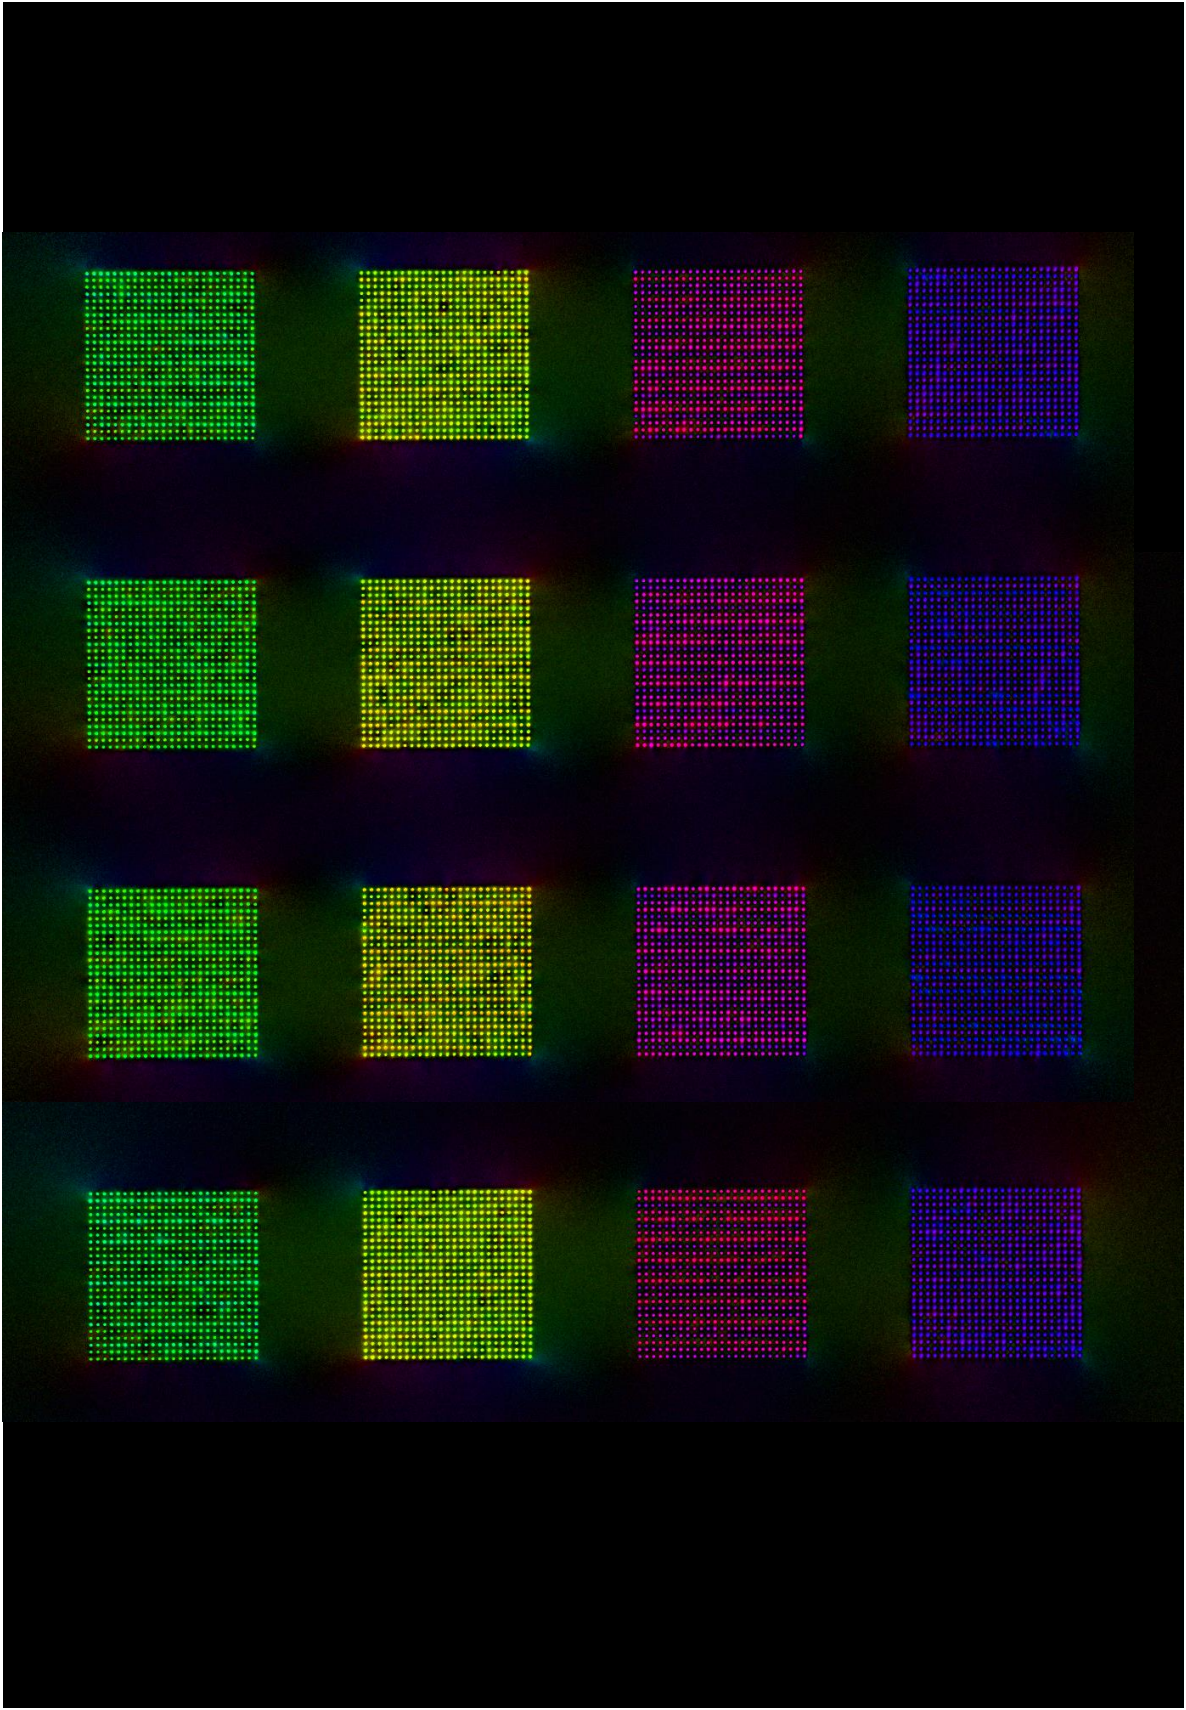

Figure 20: 8-bit dataset for encoded data of 256 classifications (Part 12).

## 7 Measurement of real data based on birefringence microscopy system.

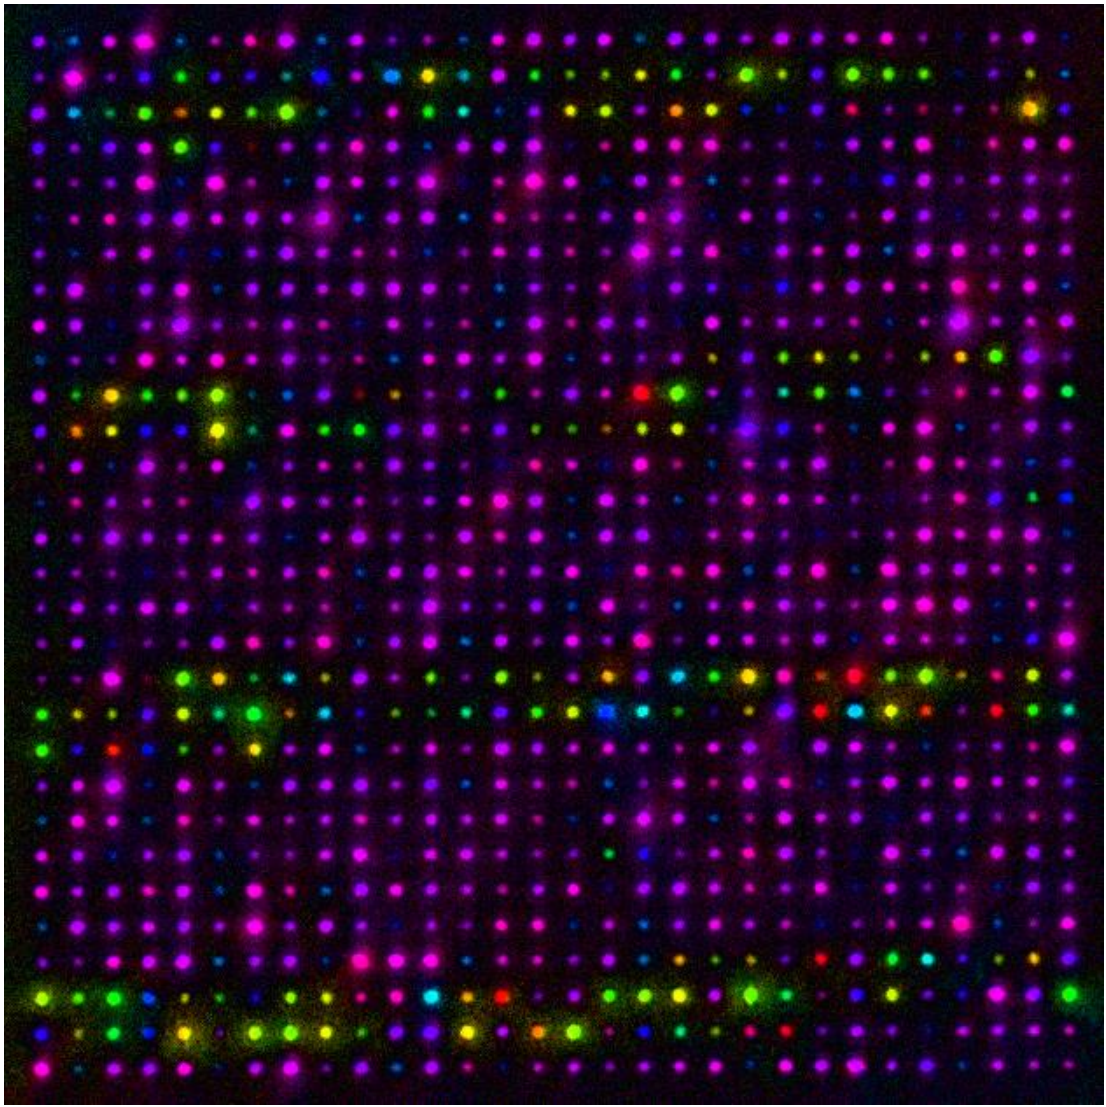

Figure 21: Display of part of the article data: “I have a dream”(part 1).

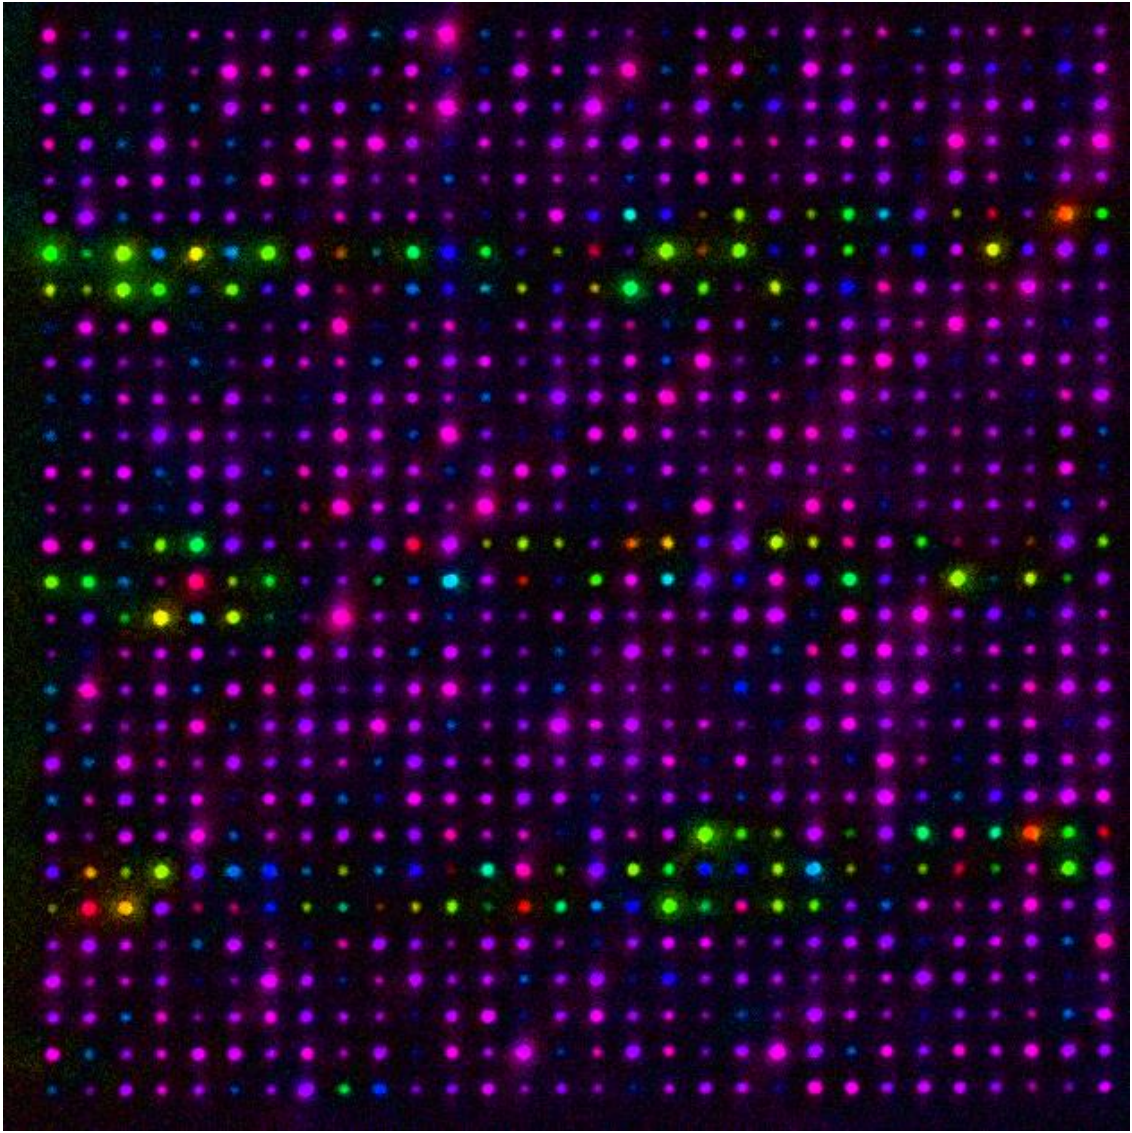

Figure 22: Display of part of the article data: “I have a dream”(part 2).

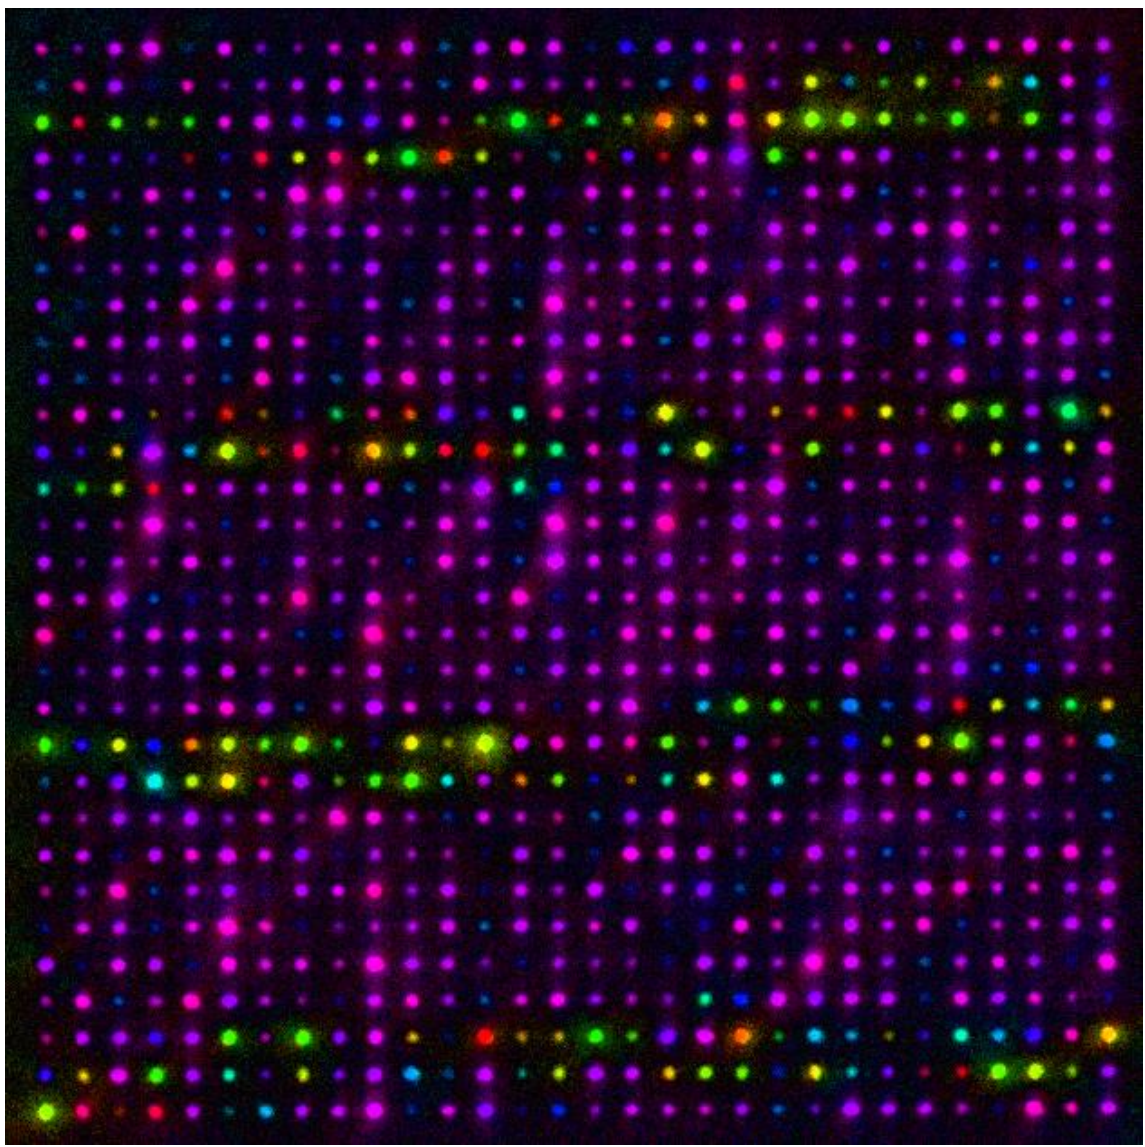

Figure 23: Display of part of the article data: “I have a dream”(part 3).

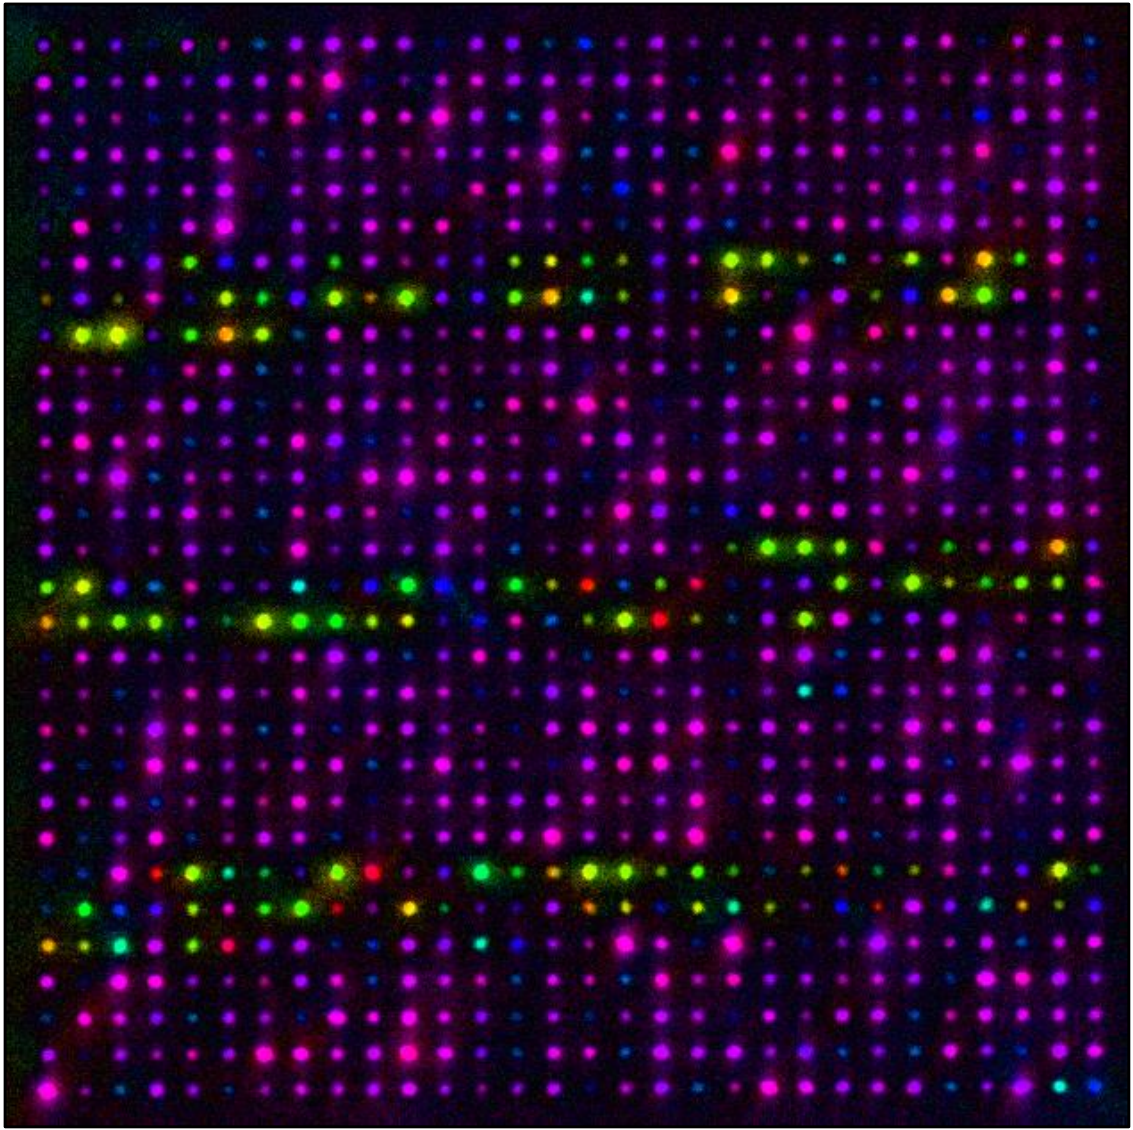

Figure 24: Display of part of the article data: “I have a dream”(part 4).

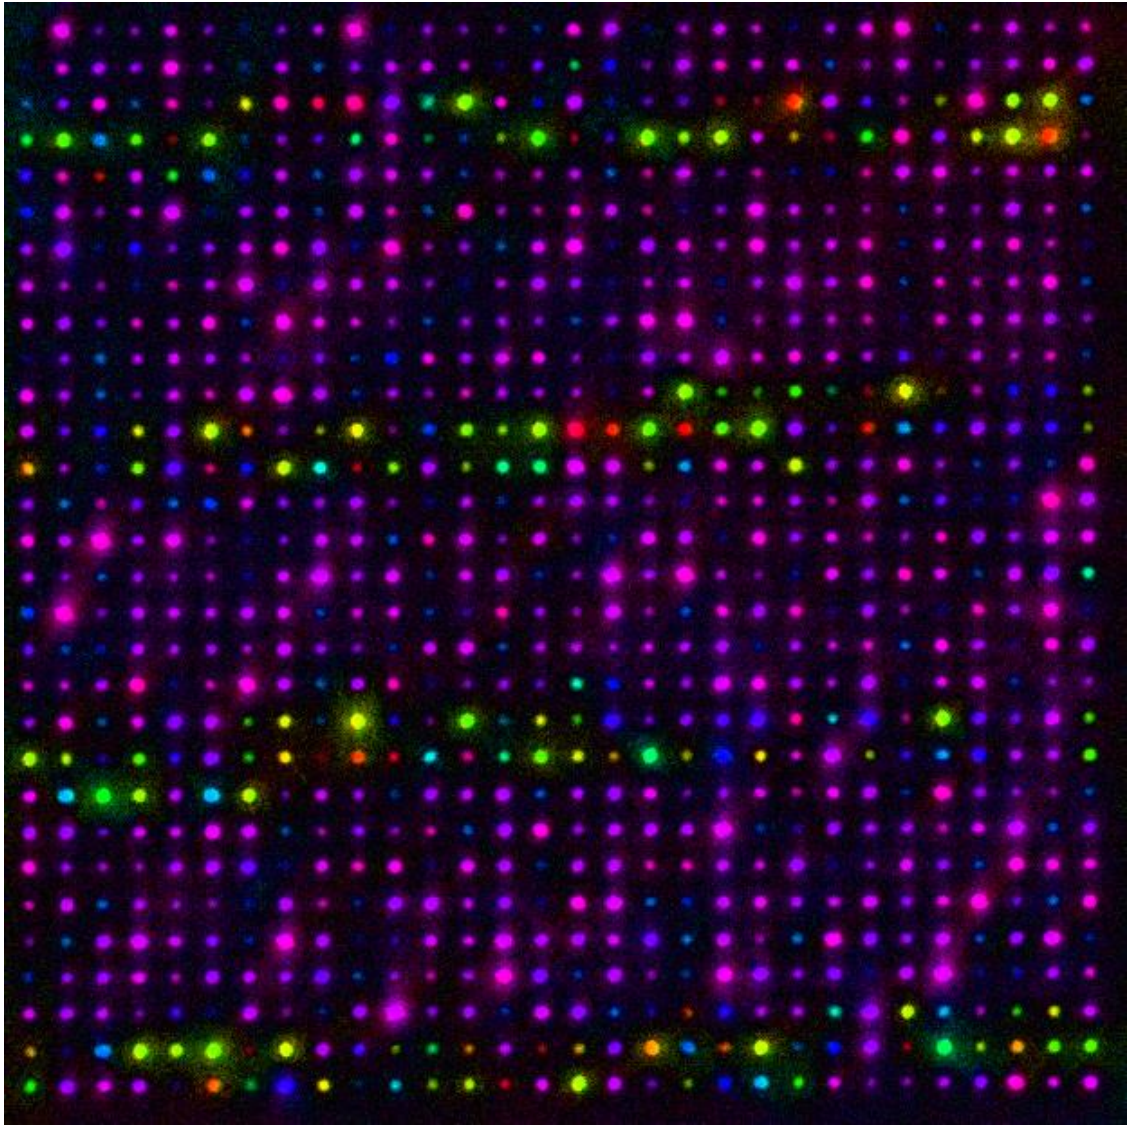

Figure 25: Display of part of the article data: “I have a dream”(part 5).

## 8 Multi-layer data simulation diagram based on real data.

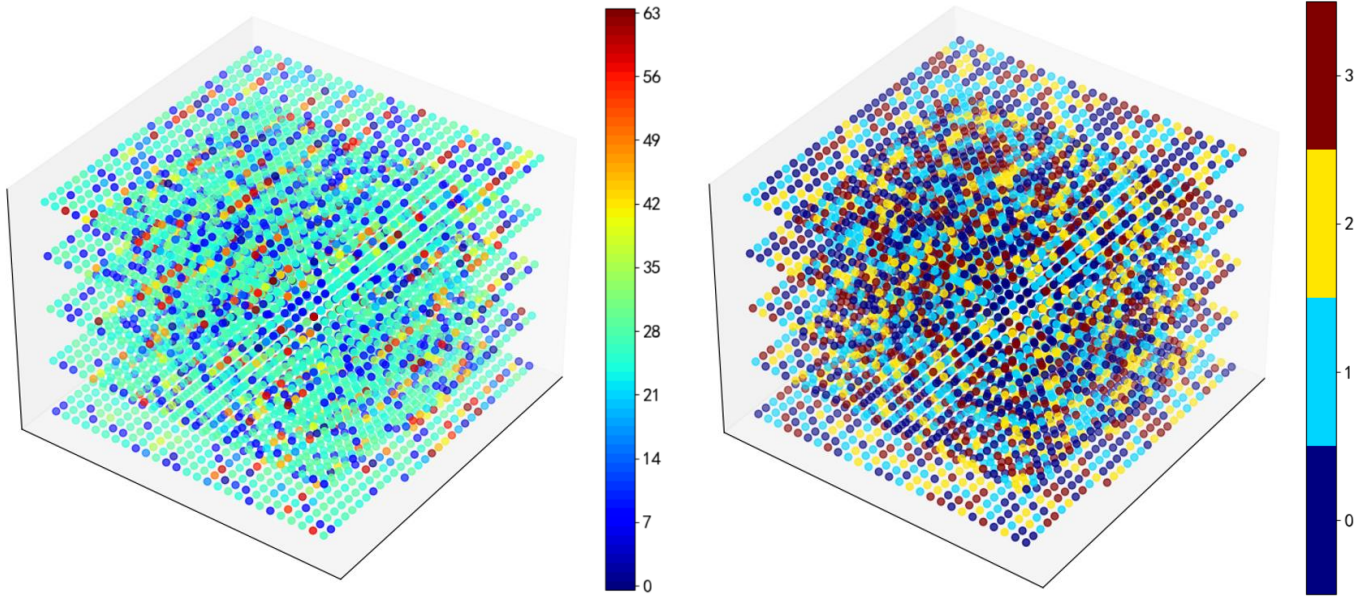

Figure 26: A program simulation demonstrating parts of Martin Luther King’s speech “I have a dream”. The data has been written in 5 layers, with 30 points per row. The data is encoded as 64 bits in the polarization angle dimension, corresponding to 64 colors of the data points (Left image); The retardance dimension is 4-bit encoded, corresponding to four sizes of data points(Right image).

## 9 Binary data represented by some data points in Figure 4

The **original data** is:

```
01110101 01110011 01110100 01101001 01100011 01100101 00101110 00100000 01001001 01110100 00100000
01100011 01100001 01101101 01100101 00100000 01100001 01110011 00100000 01100001 00100000 01101010
01101111 01111001
```

The **redundant data** is:

```
01101111 01110101 01110011 00100000 01100100 01100001 01111001 01100010
```

The corresponding article “I have a dream” in the first paragraph of the original text is “justice. It came as a joyous dayb”. The first paragraph is: Five score years ago, a great American, in whose symbolic shadow we stand today, signed the Emancipation Proclamation. This momentous decree came as a great beacon light of hope to millions of Negro slaves who had been seared in the flames of withering injustice. It came as a joyous daybreak to end the long night of their captivity. Due to the problem of incorrect writing or reading, the data of justice was restored to justicb, and it was correctly restored using the RS error correction algorithm.

## 10 The Encoding and Decoding Principle of Reed-Solomon Error Correction Algorithm.

Reed-Solomon codes are a type of error-correcting codes widely used in digital communication systems. They are designed to correct errors in data transmission by adding redundancy to the original message.

The following explains the principle of RS error correction codes from the perspective of math.

Encoding algorithm:

The encoding algorithm for Reed-Solomon codes involves two main steps: message polynomial generation and codeword polynomial generation.

Message polynomial generation: The first step is to represent the message as a polynomial of degree  $k - 1$ , where  $k$  is the number of message symbols. Let  $m(x)$  be the message polynomial, defined as:

$$m(x) = m_0 + m_1x + m_2x^2 + \cdots + m_{k-1}x^{k-1} \quad (1)$$

where  $m_i$  represents the  $i - th$  message symbol.

Codeword polynomial generation: The second step is to generate the codeword polynomial by adding redundancy to the message polynomial. The codeword polynomial is a polynomial of degree  $n - 1$ , where  $n$  is the total number of symbols in the codeword. The codeword polynomial is defined as:

$$c(x) = m(x)x^{n-k} + r(x) \quad (2)$$

where  $r(x)$  is the redundancy polynomial, which is also a polynomial of degree  $n - k - 1$ .

The redundancy polynomial is generated by performing polynomial division of a generator polynomial  $g(x)$  into the message polynomial multiplied by  $x^{n-k}$ . The generator polynomial is a fixed polynomial of degree  $r$ , where  $r$  is the number of redundancy symbols. The generator polynomial is usually chosen to be a primitive polynomial, which means that its roots are primitive elements of a finite field.

The polynomial division can be performed using the following steps:

Let  $g(x)$  be the generator polynomial, defined as:

$$g(x) = (x - \alpha_1)(x - \alpha_2) \cdots (x - \alpha_r) \quad (3)$$

where  $\alpha_1, \alpha_2, \dots, \alpha_r$  are the roots of the generator polynomial.

Multiply the message polynomial by  $x^{n-k}$  to obtain a polynomial of degree  $n - 1$ :

$$m'(x) = m(x)x^{n-k} \quad (4)$$

Perform polynomial division of  $m'(x)$  by  $g(x)$  to obtain the remainder polynomial  $r(x)$ :

$$m'(x) = q(x)g(x) + r(x) \quad (5)$$

where  $q(x)$  is the quotient polynomial.

The codeword polynomial is obtained by adding the remainder polynomial  $r(x)$  to the message polynomial multiplied by  $x^{n-k}$ :

$$c(x) = m'(x) + r(x) = m(x)x^{n-k} + r(x) \quad (6)$$

Decoding algorithm:

The decoding algorithm for RS codes involves two main steps: syndrome calculation and error correction.

Syndrome calculation: The first step is to calculate the syndrome polynomial  $s(x)$ , which is a polynomial of degree  $r - 1$ , where  $r$  is the number of redundancy symbols. The syndrome polynomial is calculated by evaluating the received polynomial  $r(x)$  at the roots of the generator polynomial  $g(x)$ :

$$s_i = r(\alpha_i) \quad i = 1, 2, \dots, r \quad (7)$$

Error correction: The second step is to correct errors in the received polynomial  $r(x)$  using the syndrome polynomial  $s(x)$ . The error correction can be performed using the Berlekamp-Massey algorithm, which is a polynomial factorization algorithm that can be used to find the error locator polynomial and the error evaluator polynomial.

The error locator polynomial  $\Lambda(x)$  is a polynomial of degree  $e$ , where  $e$  is the number of errors in the received polynomial  $r(x)$ . The error locator polynomial can be found by solving the key equation:

$$s(x)\Lambda(x) \equiv 0 \pmod{x^r} \quad (8)$$

where  $\equiv$  denotes congruence modulo  $x^r$ .

The error evaluator polynomial  $\Omega(x)$  is a polynomial of degree  $e-1$ . The error evaluator polynomial can be found by solving the following system of equations:

$$\Omega(\alpha_i)\Lambda(\alpha_i) = 1 \quad i = 1, 2, \dots, e \quad \Omega(\alpha_i)\Lambda(\alpha_i) = 0 \quad i = e+1, e+2, \dots, r \quad (9)$$

Once the error locator polynomial  $\Lambda(x)$  and the error evaluator polynomial  $\Omega(x)$  are found, the errors in the received polynomial  $r(x)$  can be corrected by calculating the error values using the following equation:

$$e_i = -\frac{r(\alpha_i)}{\Lambda'(\alpha_i)}\Omega(\alpha_i) \quad (10)$$

where  $\Lambda'(\alpha_i)$  is the derivative of the error locator polynomial evaluated at  $\alpha_i$ .

The corrected polynomial  $\hat{c}(x)$  can then be obtained by subtracting the error polynomial from the received polynomial:

$$\hat{c}(x) = r(x) - e_1(x - \alpha_1) \cdots (x - \alpha_e) \quad (11)$$

The corrected message polynomial  $\hat{m}(x)$  can be obtained by dividing the corrected polynomial  $\hat{c}(x)$  by  $x^{n-k}$ :

$$\hat{m}(x) = \frac{\hat{c}(x)}{x^{n-k}} \quad (12)$$

and extracting the first  $k$  coefficients of the resulting polynomial.
